# Supplementary material for: Effect of a magnetosphere compression on Jovian radio emissions: in situ case study using Juno data
Source: arXiv:2212.03740 source file (2023-08-10)
Supplement: Supplementary file 1 [file SI_2022JA031155.pdf]

# Supporting Information for "Effect of a magnetospheric compression on Jovian radio emissions: an in situ case study using Juno data"

C. K. Louis<sup>1,2</sup>, C. M. Jackman<sup>1</sup>, G. Hospodarsky<sup>3</sup>, A. O’Kane Hackett<sup>1,4</sup>, E. Devon-Hurley<sup>1,4</sup>, P. Zarka<sup>2,5</sup>, W. S. Kurth<sup>3</sup>, R. W. Ebert<sup>6,7</sup>, D. M. Weigt<sup>1</sup>, A. R. Fogg<sup>1</sup>, J. E. Waters<sup>8</sup>, S. McEntee<sup>1,4</sup>, J. E. P. Connerney<sup>9</sup>, P. Louarn<sup>10</sup>, S. Levin<sup>11</sup>, S. J. Bolton<sup>6</sup>

<sup>1</sup>School of Cosmic Physics, DIAS Dunsink Observatory, Dublin Institute for Advanced Studies, Dublin 15, Ireland

<sup>2</sup>Observatoire Radioastronomique de Nançay, Observatoire de Paris, Université PSL, CNRS, University Orléans, Nancay, France

<sup>3</sup>Department of Physics and Astronomy, University of Iowa, Iowa City, Iowa, USA

<sup>4</sup>School of Physics, Trinity College Dublin, Dublin, Ireland

<sup>5</sup>LESIA, Observatoire de Paris, PSL Research University, CNRS, Sorbonne Université,

<sup>6</sup>Southwest Research Institute, San Antonio, Texas, USA

<sup>7</sup>Department of Physics and Astronomy, University of Texas at San Antonio, San Antonio, Texas, USA

UPMC University, Paris 06, University Paris Diderot, Sorbonne Paris Cité, Meudon, France

<sup>8</sup>Department of Physics and Astronomy, University of Southampton, Highfield Campus, Southampton, SO17 1BJ, UK

<sup>9</sup>Space Research Corporation, Annapolis, MD

<sup>10</sup>IRAP, Université de Toulouse, CNRS, CNES, UPS, (Toulouse), France

<sup>11</sup>Jet Propulsion Laboratory, Pasadena, California, USA

## Contents of this file:

1. Tables S1 to S2
2. Files F1 and F2
3. Figures S1 to S4

## Introduction

This Supporting Information contains magnetosphere boundaries crossings (Tables S1 and S2) and original csv files (Files F1 and F2), 3D projection of the magnetosphere boundaries crossings (Figure S1), outputs of Tao et al. (2005)’s model (Figures S2 and S3), and timeseries of the narrowband Kilometric emission separated by frequency channel, for the interval studied in the main article. (Figure S4).

Tables S1, S2 and Files F1, F2 are directly downloadable at:  
<https://doi.org/10.5281/zenodo.7304516> (Louis et al., 2022).

---

**Table S1 – List of Magnetopause boundary crossings from Juno/Waves and Juno/MAG measurements**

All this information is also available directly in the file:  
*boundary\_crossings\_characteristics\_list.csv* (File F1).

*Table S 1: List of magnetopause crossings, as measured by Juno/Waves and Juno/MAG. For each crossing, number of the crossing (MP#), day of the year (DOY), date (day/month/year format) and time (hours:minutes format) are indicated, as well as the boundary crossed (magnetopause in this case), the direction of the crossing (in: from the magnetosphere to the magnetosheath; out: from the magnetosheath to the magnetosphere). The column “Notes” indicates whether the magnetopause has potentially not been completely crossed (see Fig. 1c). Position of the crossings are given in the Cartesian Jupiter-Heliospheric (JH) and the International Astronomical Union (IAU) coordinate systems, and IAU spherical coordinates system. Finally, the dynamic pressure of the solar wind, and the standoff distance of the magnetopause and the bow shock, derived from the model of Joy et al. (2002), are given in the last three columns. Note that the list of crossings up to 2016-11-26 was provided by Hospodarsky et al. (2017).*

## Supporting Information for “Effect of a magnetosphere compression on Jovian radio emissions: an in situ case study using Juno data”

- (1) JSS coordinate system: this coordinate system is defined such that X points towards the Sun, the Z axis is along the Jovian spin axis, positive in the direction of angular momentum, and Y completes the righthanded set (positive towards dusk).  
 (2) IAU coordinate system: this coordinate system is defined such that Z-axis is along the Jovian spin axis, X-axis is defined by 0° latitude on the System III longitude  $\lambda_{III} = 0^\circ$  (prime meridian). The Y-axis completes the orthogonal right-handed system.  
 (3) Values determined using the Joy et al. (2002)'s model.  
 Note: the nan values in the 'standoff distance' columns are given when the bow shock standoff distance calculated from the Joy et al. (2002) model is smaller than that of the magnetopause (non-physical).

| #    | Day of Year | Date<br>(day/month/year) | Time<br>(HH:MM) | Boundary     | in/out | Notes                   | x<br>(JSS <sup>1</sup> ) | y<br>(JSS <sup>1</sup> ) | z<br>(JSS <sup>1</sup> ) | x<br>(IAU <sup>2</sup> ) | y<br>(IAU <sup>2</sup> ) | z<br>(IAU <sup>2</sup> ) | r<br>(IAU <sup>2</sup> ) | $\theta$<br>(IAU <sup>2</sup> ) | $\phi$<br>(IAU <sup>2</sup> ) | Dynamic<br>Pressure <sup>3</sup><br>(nPa) | Magnetopause<br>Standoff<br>Distance <sup>3</sup><br>(Jovian radius) | Bow Shock<br>Standoff<br>Distance <sup>3</sup><br>(Jovian radius) |
|------|-------------|--------------------------|-----------------|--------------|--------|-------------------------|--------------------------|--------------------------|--------------------------|--------------------------|--------------------------|--------------------------|--------------------------|---------------------------------|-------------------------------|-------------------------------------------|----------------------------------------------------------------------|-------------------------------------------------------------------|
| MP1  | 177         | 25/06/2016               | 21:20           | magnetopause | in     |                         | 5.744                    | -110.859                 | 25.498                   | -18.942                  | -109.380                 | 25.498                   | 113.899                  | 1.345                           | -1.742                        | 0.067                                     | 84.300                                                               | 109.100                                                           |
| MP2  | 180         | 28/06/2016               | 22:27           | magnetopause | out    |                         | 3.907                    | -81.666                  | 20.808                   | -51.758                  | 63.291                   | 20.808                   | 84.366                   | 1.322                           | 2.256                         | 0.267                                     | 64.900                                                               | 77.300                                                            |
| MP3  | 181         | 29/06/2016               | 08:40           | magnetopause | in     |                         | 3.659                    | -77.352                  | 20.096                   | -35.740                  | 68.697                   | 20.096                   | 80.003                   | 1.317                           | 2.051                         | 0.323                                     | 62.300                                                               | 72.500                                                            |
| MP4  | 181         | 29/06/2016               | 09:23           | magnetopause | out    |                         | 3.640                    | -77.033                  | 20.043                   | -0.379                   | 77.118                   | 20.043                   | 79.681                   | 1.317                           | 1.576                         | 0.328                                     | 62.200                                                               | 72.100                                                            |
| MP5  | 181         | 29/06/2016               | 11:07           | magnetopause | in     |                         | 3.600                    | -76.324                  | 19.926                   | 66.287                   | 38.005                   | 19.926                   | 78.964                   | 1.316                           | 0.521                         | 0.338                                     | 61.800                                                               | 71.300                                                            |
| MP6  | 181         | 29/06/2016               | 17:12           | magnetopause | out    |                         | 3.453                    | -73.719                  | 19.492                   | -72.486                  | 13.864                   | 19.492                   | 76.331                   | 1.313                           | 2.953                         | 0.378                                     | 60.300                                                               | 68.400                                                            |
| MP7  | 181         | 29/06/2016               | 23:41           | magnetopause | in     |                         | 3.297                    | -70.906                  | 19.020                   | 28.193                   | -65.143                  | 19.020                   | 73.486                   | 1.309                           | -1.162                        | 0.426                                     | 58.700                                                               | 65.300                                                            |
| MP8  | 196         | 14/07/2016               | 21:18           | magnetopause | out    |                         | 2.047                    | -80.750                  | -14.404                  | 13.911                   | -79.569                  | -14.404                  | 82.050                   | 1.747                           | -1.398                        | 0.307                                     | 63.000                                                               | 73.800                                                            |
| MP9  | 197         | 15/07/2016               | 07:16           | magnetopause | in     |                         | 2.046                    | -82.463                  | -14.334                  | 14.632                   | -81.180                  | -14.334                  | 83.724                   | 1.743                           | -1.392                        | 0.287                                     | 63.900                                                               | 75.500                                                            |
| MP10 | 197         | 15/07/2016               | 17:06           | magnetopause | out    | maybe not fully crossed | 2.042                    | -84.100                  | -14.254                  | 19.695                   | -81.787                  | -14.254                  | 85.324                   | 1.739                           | -1.334                        | 0.268                                     | 64.800                                                               | 77.200                                                            |
| MP11 | 197         | 15/07/2016               | 19:11           | magnetopause | in     | maybe not fully crossed | 2.041                    | -84.440                  | -14.235                  | -74.597                  | -39.618                  | -14.235                  | 85.655                   | 1.738                           | -2.653                        | 0.264                                     | 65.000                                                               | 77.500                                                            |
| MP12 | 198         | 16/07/2016               | 23:07           | magnetopause | out    |                         | 2.012                    | -88.741                  | -13.949                  | 8.310                    | -88.374                  | -13.949                  | 89.853                   | 1.727                           | -1.477                        | 0.221                                     | 67.400                                                               | 81.900                                                            |
| MP13 | 201         | 19/07/2016               | 17:26           | magnetopause | in     |                         | 1.851                    | -97.302                  | -13.015                  | 84.863                   | 47.638                   | -13.015                  | 98.186                   | 1.704                           | 0.512                         | 0.155                                     | 72.400                                                               | 90.500                                                            |
| MP14 | 201         | 19/07/2016               | 20:43           | magnetopause | out    |                         | 1.841                    | -97.677                  | -12.960                  | -2.727                   | -97.656                  | -12.960                  | 98.550                   | 1.703                           | -1.599                        | 0.152                                     | 72.600                                                               | 90.900                                                            |
| MP15 | 202         | 20/07/2016               | 09:18           | magnetopause | in     |                         | 1.800                    | -99.042                  | -12.747                  | -98.088                  | 13.830                   | -12.747                  | 99.876                   | 1.699                           | 3.002                         | 0.144                                     | 73.400                                                               | 92.200                                                            |
| MP16 | 202         | 20/07/2016               | 19:16           | magnetopause | out    |                         | 1.765                    | -100.068                 | -12.572                  | -99.175                  | 13.455                   | -12.572                  | 100.870                  | 1.696                           | 3.007                         | 0.137                                     | 74.000                                                               | 93.300                                                            |
| MP17 | 203         | 21/07/2016               | 01:49           | magnetopause | in     |                         | 1.740                    | -100.726                 | -12.453                  | 40.141                   | -92.398                  | -12.453                  | 101.508                  | 1.694                           | -1.161                        | 0.134                                     | 74.400                                                               | 93.900                                                            |
| MP18 | 203         | 21/07/2016               | 02:02           | magnetopause | out    |                         | 1.739                    | -100.742                 | -12.450                  | 30.191                   | -96.127                  | -12.450                  | 101.523                  | 1.694                           | -1.266                        | 0.134                                     | 74.400                                                               | 93.900                                                            |
| MP19 | 204         | 22/07/2016               | 14:31           | magnetopause | in     |                         | 1.592                    | -104.049                 | -11.751                  | 75.485                   | 71.629                   | -11.751                  | 104.723                  | 1.683                           | 0.759                         | 0.116                                     | 76.400                                                               | 97.100                                                            |
| MP20 | 205         | 23/07/2016               | 14:06           | magnetopause | out    |                         | 1.485                    | -105.895                 | -11.265                  | -3.553                   | -105.845                 | -11.265                  | 106.502                  | 1.677                           | -1.604                        | 0.107                                     | 77.500                                                               | 98.900                                                            |
| MP21 | 205         | 23/07/2016               | 19:54           | magnetopause | in     |                         | 1.458                    | -106.317                 | -11.142                  | 58.702                   | 88.653                   | -11.142                  | 106.909                  | 1.675                           | 0.986                         | 0.105                                     | 77.800                                                               | 99.300                                                            |
| MP22 | 206         | 24/07/2016               | 18:47           | magnetopause | out    |                         | 1.345                    | -107.841                 | -10.644                  | 66.801                   | -84.670                  | -10.644                  | 108.373                  | 1.669                           | -0.903                        | 0.099                                     | 78.700                                                               | 100.700                                                           |
| MP23 | 207         | 25/07/2016               | 01:12           | magnetopause | in     |                         | 1.312                    | -108.234                 | -10.501                  | 27.056                   | 104.805                  | -10.501                  | 108.749                  | 1.668                           | 1.318                         | 0.097                                     | 78.900                                                               | 101.100                                                           |
| MP24 | 207         | 25/07/2016               | 14:33           | magnetopause | out    |                         | 1.242                    | -109.004                 | -10.196                  | 68.413                   | -84.872                  | -10.196                  | 109.487                  | 1.664                           | -0.892                        | 0.094                                     | 79.400                                                               | 101.800                                                           |
| MP25 | 212         | 30/07/2016               | 00:22           | magnetopause | in     |                         | 0.638                    | -112.778                 | -7.597                   | 32.828                   | 107.896                  | -7.597                   | 113.035                  | 1.638                           | 1.275                         | 0.081                                     | 81.500                                                               | 105.000                                                           |
| MP26 | 214         | 01/08/2016               | 19:36           | magnetopause | out    |                         | 0.225                    | -113.113                 | -5.798                   | -101.461                 | 50.002                   | -5.798                   | 113.262                  | 1.622                           | 2.684                         | 0.081                                     | 81.400                                                               | 104.900                                                           |
| MP27 | 214         | 01/08/2016               | 20:57           | magnetopause | in     |                         | 0.217                    | -113.103                 | -5.762                   | -30.039                  | 109.042                  | -5.762                   | 113.250                  | 1.622                           | 1.840                         | 0.081                                     | 81.400                                                               | 104.900                                                           |
| MP28 | 214         | 01/08/2016               | 21:55           | magnetopause | out    | maybe not fully crossed | 0.210                    | -113.096                 | -5.734                   | 40.291                   | 105.676                  | -5.734                   | 113.242                  | 1.621                           | 1.207                         | 0.081                                     | 81.400                                                               | 104.900                                                           |
| MP29 | 215         | 02/08/2016               | 08:13           | magnetopause | in     | maybe not fully crossed | 0.146                    | -112.999                 | -5.449                   | 65.915                   | 91.782                   | -5.449                   | 113.130                  | 1.619                           | 0.948                         | 0.082                                     | 81.300                                                               | 104.700                                                           |
| MP30 | 215         | 02/08/2016               | 10:50           | magnetopause | out    | maybe not fully crossed | 0.130                    | -112.969                 | -5.378                   | 87.309                   | -71.687                  | -5.378                   | 113.097                  | 1.618                           | -0.687                        | 0.082                                     | 81.300                                                               | 104.700                                                           |
| MP31 | 215         | 02/08/2016               | 13:59           | magnetopause | in     |                         | 0.110                    | -112.929                 | -5.290                   | -101.716                 | -49.060                  | -5.290                   | 113.053                  | 1.618                           | -2.692                        | 0.082                                     | 81.300                                                               | 104.600                                                           |
| MP32 | 215         | 02/08/2016               | 22:12           | magnetopause | out    |                         | 0.059                    | -112.810                 | -5.063                   | -0.935                   | -112.806                 | -5.063                   | 112.923                  | 1.616                           | -1.579                        | 0.083                                     | 81.100                                                               | 104.500                                                           |
| MP33 | 215         | 02/08/2016               | 22:49           | magnetopause | in     |                         | 0.055                    | -112.799                 | -5.045                   | -47.057                  | -102.515                 | -5.045                   | 112.912                  | 1.615                           | -2.001                        | 0.083                                     | 81.100                                                               | 104.500                                                           |
| MP34 | 219         | 06/08/2016               | 19:56           | magnetopause | out    |                         | -0.501                   | -109.731                 | -2.393                   | -35.722                  | 103.755                  | -2.393                   | 109.758                  | 1.593                           | 1.902                         | 0.098                                     | 78.800                                                               | 100.900                                                           |
| MP35 | 219         | 06/08/2016               | 23:50           | magnetopause | in     |                         | -0.523                   | -109.533                 | -2.280                   | 91.792                   | -59.766                  | -2.280                   | 109.558                  | 1.592                           | -0.577                        | 0.099                                     | 78.700                                                               | 100.700                                                           |
| MP36 | 220         | 07/08/2016               | 01:20           | magnetopause | out    |                         | -0.531                   | -109.455                 | -2.236                   | 4.819                    | -109.350                 | -2.236                   | 109.479                  | 1.591                           | -1.527                        | 0.099                                     | 78.600                                                               | 100.600                                                           |
| MP37 | 221         | 08/08/2016               | 08:44           | magnetopause | in     |                         | -0.707                   | -107.633                 | -1.321                   | -90.303                  | -58.573                  | -1.321                   | 107.644                  | 1.583                           | -2.566                        | 0.108                                     | 77.400                                                               | 98.700                                                            |
| MP38 | 221         | 08/08/2016               | 14:35           | magnetopause | out    |                         | -0.739                   | -107.253                 | -1.150                   | 107.225                  | 2.583                    | -1.150                   | 107.262                  | 1.582                           | 0.024                         | 0.110                                     | 77.100                                                               | 98.300                                                            |
| MP39 | 221         | 08/08/2016               | 15:26           | magnetopause | in     |                         | -0.743                   | -107.198                 | -1.126                   | 93.898                   | -51.721                  | -1.126                   | 107.207                  | 1.581                           | -0.503                        | 0.111                                     | 77.100                                                               | 98.200                                                            |
| MP40 | 221         | 08/08/2016               | 15:38           | magnetopause | out    |                         | -0.744                   | -107.181                 | -1.118                   | 84.560                   | -65.864                  | -1.118                   | 107.190                  | 1.581                           | -0.662                        | 0.111                                     | 77.100                                                               | 98.200                                                            |
| MP41 | 224         | 11/08/2016               | 17:12           | magnetopause | in     |                         | -1.106                   | -101.187                 | 1.036                    | -100.955                 | 6.932                    | 1.036                    | 101.198                  | 1.561                           | 3.073                         | 0.146                                     | 73.100                                                               | 91.800                                                            |
| MP42 | 224         | 11/08/2016               | 23:25           | magnetopause | out    |                         | -1.133                   | -100.572                 | 1.219                    | 63.800                   | -77.754                  | 1.219                    | 100.586                  | 1.559                           | -0.884                        | 0.151                                     | 72.700                                                               | 91.100                                                            |
| MP43 | 225         | 12/08/2016               | 03:56           | magnetopause | in     |                         | -1.152                   | -100.118                 | 1.350                    | -83.149                  | 55.779                   | 1.350                    | 100.134                  | 1.557                           | 2.551                         | 0.154                                     | 72.500                                                               | 90.700                                                            |
| MP44 | 225         | 12/08/2016               | 10:05           | magnetopause | out    |                         | -1.178                   | -99.482                  | 1.530                    | 21.476                   | -97.143                  | 1.530                    | 99.500                   | 1.555                           | -1.353                        | 0.158                                     | 72.100                                                               | 90.000                                                            |
| MP45 | 225         | 12/08/2016               | 12:39           | magnetopause | in     |                         | -1.188                   | -99.210                  | 1.605                    | -98.059                  | -15.116                  | 1.605                    | 99.230                   | 1.555                           | -2.989                        | 0.160                                     | 71.900                                                               | 89.700                                                            |
| MP46 | 225         | 12/08/2016               | 21:11           | magnetopause | out    |                         | -1.222                   | -98.293                  | 1.853                    | -48.482                  | -85.514                  | 1.853                    | 98.318                   | 1.552                           | -2.087                        | 0.167                                     | 71.300                                                               | 88.700                                                            |
| MP47 | 225         | 12/08/2016               | 23:55           | magnetopause | in     | maybe not fully crossed | -1.233                   | -97.990                  | 1.933                    | -75.835                  | 62.070                   | 1.933                    | 98.017                   | 1.551                           | 2.456                         | 0.169                                     | 71.100                                                               | 88.400                                                            |
| MP48 | 250         | 06/09/2016               | 11:02           | magnetopause | out    |                         | -3.699                   | -81.053                  | -15.622                  | 5.976                    | 80.917                   | -15.622                  | 82.628                   | 1.761                           | 1.497                         | 0.346                                     | 61.500                                                               | 70.700                                                            |

# Supporting Information for “Effect of a magnetosphere compression on Jovian radio emissions: an in situ case study using Juno data”

|       |     |            |       |              |     |                         |         |          |         |          |          |         |         |       |        |       |        |         |
|-------|-----|------------|-------|--------------|-----|-------------------------|---------|----------|---------|----------|----------|---------|---------|-------|--------|-------|--------|---------|
| MP49  | 250 | 06/09/2016 | 21:47 | magnetopause | in  |                         | -3.831  | -82.875  | -15.568 | 46.574   | 68.657   | -15.568 | 84.412  | 1.756 | 0.975  | 0.322 | 62.400 | 72.500  |
| MP50  | 251 | 07/09/2016 | 03:15 | magnetopause | out |                         | -3.898  | -83.780  | -15.535 | -67.549  | -49.712  | -15.535 | 85.297  | 1.754 | -2.507 | 0.311 | 62.800 | 73.400  |
| MP51  | 252 | 08/09/2016 | 23:56 | magnetopause | in  | maybe not fully crossed | -4.429  | -90.473  | -15.151 | 73.106   | 53.483   | -15.151 | 91.839  | 1.737 | 0.632  | 0.240 | 66.300 | 80.000  |
| MP52  | 258 | 14/09/2016 | 22:50 | magnetopause | out | maybe not fully crossed | -5.973  | -105.315 | -12.889 | -32.115  | -100.477 | -12.889 | 106.269 | 1.692 | -1.880 | 0.133 | 74.500 | 94.100  |
| MP53  | 260 | 16/09/2016 | 21:51 | magnetopause | in  | maybe not fully crossed | -6.421  | -108.331 | -11.899 | 105.940  | -23.530  | -11.899 | 109.172 | 1.680 | -0.219 | 0.118 | 76.200 | 96.800  |
| MP54  | 263 | 19/09/2016 | 07:05 | magnetopause | out |                         | -6.918  | -110.884 | -10.569 | 36.375   | 104.976  | -10.569 | 111.601 | 1.666 | 1.237  | 0.107 | 77.600 | 98.900  |
| MP55  | 263 | 19/09/2016 | 20:41 | magnetopause | in  | maybe not fully crossed | -7.028  | -111.315 | -10.237 | 52.688   | -98.307  | -10.237 | 112.005 | 1.662 | -1.079 | 0.105 | 77.800 | 99.300  |
| MP56  | 264 | 20/09/2016 | 07:05 | magnetopause | out | maybe not fully crossed | -7.110  | -111.601 | -9.978  | 20.096   | -110.006 | -9.978  | 112.271 | 1.660 | -1.390 | 0.104 | 77.900 | 99.500  |
| MP57  | 264 | 20/09/2016 | 13:20 | magnetopause | in  | maybe not fully crossed | -7.159  | -111.753 | -9.820  | 66.373   | 90.192   | -9.820  | 112.412 | 1.658 | 0.936  | 0.104 | 78.000 | 99.600  |
| MP58  | 266 | 22/09/2016 | 02:28 | magnetopause | out |                         | -7.430  | -112.381 | -8.862  | -92.850  | 63.746   | -8.862  | 112.974 | 1.649 | 2.540  | 0.102 | 78.200 | 100.000 |
| MP59  | 266 | 22/09/2016 | 09:40 | magnetopause | in  |                         | -7.479  | -112.446 | -8.672  | -46.596  | -102.610 | -8.672  | 113.028 | 1.648 | -1.997 | 0.102 | 78.200 | 100.000 |
| MP60  | 267 | 23/09/2016 | 18:09 | magnetopause | out |                         | -7.685  | -112.516 | -7.796  | -94.289  | 61.874   | -7.796  | 113.047 | 1.640 | 2.561  | 0.102 | 78.200 | 99.900  |
| MP61  | 267 | 23/09/2016 | 21:05 | magnetopause | in  |                         | -7.702  | -112.504 | -7.717  | 85.194   | 73.881   | -7.717  | 113.031 | 1.639 | 0.714  | 0.102 | 78.200 | 99.900  |
| MP62  | 272 | 28/09/2016 | 01:35 | magnetopause | out | maybe not fully crossed | -8.157  | -110.253 | -4.852  | 110.223  | -8.550   | -4.852  | 110.661 | 1.615 | -0.077 | 0.116 | 76.400 | 97.200  |
| MP63  | 273 | 29/09/2016 | 13:05 | magnetopause | in  | maybe not fully crossed | -8.245  | -108.587 | -3.797  | -92.248  | 57.873   | -3.797  | 108.965 | 1.606 | 2.581  | 0.125 | 75.300 | 95.300  |
| MP64  | 274 | 30/09/2016 | 13:17 | magnetopause | out |                         | -8.281  | -107.181 | -3.070  | 106.268  | -16.230  | -3.070  | 107.544 | 1.599 | -0.152 | 0.134 | 74.400 | 93.800  |
| MP65  | 274 | 30/09/2016 | 16:36 | magnetopause | in  |                         | -8.284  | -106.969 | -2.969  | -68.376  | -82.678  | -2.969  | 107.331 | 1.598 | -2.262 | 0.135 | 74.200 | 93.600  |
| MP66  | 275 | 01/10/2016 | 03:54 | magnetopause | out |                         | -8.291  | -106.217 | -2.625  | -106.533 | 1.259    | -2.625  | 106.573 | 1.595 | 3.130  | 0.140 | 73.800 | 92.800  |
| MP67  | 275 | 01/10/2016 | 05:40 | magnetopause | in  |                         | -8.292  | -106.096 | -2.571  | -46.395  | 95.774   | -2.571  | 106.451 | 1.595 | 2.022  | 0.141 | 73.700 | 92.700  |
| MP68  | 275 | 01/10/2016 | 17:48 | magnetopause | out |                         | -8.294  | -105.224 | -2.201  | 86.952   | 59.835   | -2.201  | 105.573 | 1.592 | 0.603  | 0.146 | 73.100 | 91.800  |
| MP69  | 275 | 01/10/2016 | 21:44 | magnetopause | in  |                         | -8.293  | -104.931 | -2.081  | -31.710  | -100.368 | -2.081  | 105.279 | 1.591 | -1.877 | 0.148 | 72.900 | 91.500  |
| MP70  | 276 | 02/10/2016 | 01:04 | magnetopause | out |                         | -8.292  | -104.676 | -1.979  | -69.659  | 78.572   | -1.979  | 105.023 | 1.590 | 2.296  | 0.150 | 72.800 | 91.200  |
| MP71  | 278 | 04/10/2016 | 04:36 | magnetopause | in  |                         | -8.216  | -100.152 | -0.395  | 44.782   | 89.958   | -0.395  | 100.489 | 1.575 | 1.109  | 0.183 | 70.000 | 86.500  |
| MP72  | 312 | 07/11/2016 | 23:46 | magnetopause | out |                         | -13.573 | -105.565 | -14.122 | 104.790  | 18.636   | -14.121 | 107.367 | 1.703 | 0.176  | 0.157 | 72.200 | 90.200  |
| MP73  | 313 | 08/11/2016 | 09:02 | magnetopause | in  | maybe not fully crossed | -13.702 | -106.143 | -13.934 | 88.132   | 60.719   | -13.934 | 107.927 | 1.700 | 0.603  | 0.153 | 72.500 | 90.700  |
| MP74  | 313 | 08/11/2016 | 11:31 | magnetopause | out | maybe not fully crossed | -13.736 | -106.294 | -13.883 | 59.754   | -88.975  | -13.883 | 108.073 | 1.700 | -0.979 | 0.152 | 72.600 | 90.900  |
| MP75  | 314 | 09/11/2016 | 17:32 | magnetopause | in  |                         | -14.130 | -107.917 | -13.242 | 47.221   | -98.061  | -13.242 | 109.641 | 1.692 | -1.122 | 0.144 | 73.400 | 92.200  |
| MP76  | 314 | 09/11/2016 | 18:09 | magnetopause | out |                         | -14.138 | -107.950 | -13.228 | 2.909    | -108.833 | -13.228 | 109.673 | 1.692 | -1.544 | 0.143 | 73.400 | 92.300  |
| MP77  | 318 | 13/11/2016 | 08:28 | magnetopause | in  |                         | -15.048 | -110.776 | -11.167 | 105.040  | 38.267   | -11.167 | 112.350 | 1.670 | 0.349  | 0.130 | 74.700 | 94.400  |
| MP78  | 318 | 13/11/2016 | 15:08 | magnetopause | out | maybe not fully crossed | -15.104 | -110.885 | -10.996 | -83.428  | 74.588   | -10.996 | 112.448 | 1.669 | 2.412  | 0.130 | 74.800 | 94.500  |
| MP79  | 318 | 13/11/2016 | 19:55 | magnetopause | in  |                         | -15.143 | -110.952 | -10.873 | 92.736   | -62.767  | -10.873 | 112.508 | 1.668 | -0.595 | 0.130 | 74.800 | 94.500  |
| MP80  | 318 | 13/11/2016 | 21:40 | magnetopause | out |                         | -15.156 | -110.975 | -10.828 | -14.752  | -111.030 | -10.828 | 112.528 | 1.667 | -1.703 | 0.130 | 74.800 | 94.600  |
| MP81  | 319 | 14/11/2016 | 00:45 | magnetopause | in  |                         | -15.181 | -111.013 | -10.748 | -97.608  | 55.017   | -10.748 | 112.560 | 1.666 | 2.628  | 0.130 | 74.800 | 94.600  |
| MP82  | 319 | 14/11/2016 | 05:04 | magnetopause | out | maybe not fully crossed | -15.214 | -111.060 | -10.634 | 111.357  | -12.861  | -10.634 | 112.600 | 1.665 | -0.115 | 0.130 | 74.800 | 94.600  |
| MP83  | 319 | 14/11/2016 | 10:55 | magnetopause | in  | maybe not fully crossed | -15.257 | -111.113 | -10.481 | -88.166  | 69.322   | -10.481 | 112.644 | 1.664 | 2.475  | 0.130 | 74.800 | 94.600  |
| MP84  | 324 | 19/11/2016 | 06:12 | magnetopause | out |                         | -15.780 | -109.713 | -7.237  | 21.973   | -108.642 | -7.237  | 111.078 | 1.636 | -1.371 | 0.141 | 73.600 | 92.600  |
| MP85  | 324 | 19/11/2016 | 11:24 | magnetopause | in  |                         | -15.787 | -109.537 | -7.080  | -1.939   | 110.651  | -7.080  | 110.894 | 1.635 | 1.588  | 0.143 | 73.500 | 92.400  |
| MP86  | 326 | 21/11/2016 | 22:39 | magnetopause | out | maybe not fully crossed | -15.755 | -106.851 | -5.276  | -22.212  | 105.698  | -5.276  | 108.136 | 1.620 | 1.778  | 0.161 | 71.800 | 89.500  |
| MP87  | 329 | 24/11/2016 | 04:01 | magnetopause | in  |                         | -15.545 | -103.291 | -3.595  | 87.940   | -56.368  | -3.595  | 104.516 | 1.605 | -0.570 | 0.188 | 69.600 | 85.800  |
| MP88  | 330 | 25/11/2016 | 12:22 | magnetopause | out |                         | -15.322 | -100.577 | -2.555  | -59.031  | -82.861  | -2.555  | 101.770 | 1.596 | -2.190 | 0.211 | 68.100 | 83.100  |
| MP89  | 330 | 25/11/2016 | 12:54 | magnetopause | in  |                         | -15.318 | -100.524 | -2.536  | -84.916  | -55.938  | -2.536  | 101.716 | 1.596 | -2.559 | 0.211 | 68.100 | 83.100  |
| MP90  | 330 | 25/11/2016 | 13:13 | magnetopause | out |                         | -15.315 | -100.494 | -2.525  | -94.721  | -36.899  | -2.525  | 101.686 | 1.596 | -2.770 | 0.212 | 68.000 | 83.000  |
| MP91  | 330 | 25/11/2016 | 13:16 | magnetopause | in  |                         | -15.315 | -100.494 | -2.525  | -94.721  | -36.899  | -2.525  | 101.686 | 1.596 | -2.770 | 0.212 | 68.000 | 83.000  |
| MP92  | 330 | 25/11/2016 | 13:29 | magnetopause | out |                         | -15.313 | -100.471 | -2.517  | -99.330  | -21.504  | -2.517  | 101.662 | 1.596 | -2.928 | 0.212 | 68.000 | 83.000  |
| MP93  | 330 | 25/11/2016 | 14:40 | magnetopause | in  |                         | -15.303 | -100.364 | -2.480  | -87.832  | 50.919   | -2.480  | 101.555 | 1.595 | 2.616  | 0.213 | 68.000 | 82.900  |
| MP94  | 330 | 25/11/2016 | 14:52 | magnetopause | out |                         | -15.302 | -100.349 | -2.474  | -81.969  | 59.877   | -2.474  | 101.539 | 1.595 | 2.511  | 0.213 | 68.000 | 82.900  |
| MP95  | 330 | 25/11/2016 | 17:40 | magnetopause | in  |                         | -15.279 | -100.087 | -2.382  | 76.319   | 66.531   | -2.382  | 101.275 | 1.594 | 0.717  | 0.215 | 67.800 | 82.600  |
| MP96  | 330 | 25/11/2016 | 20:44 | magnetopause | out | maybe not fully crossed | -15.252 | -99.799  | -2.282  | 33.269   | -95.318  | -2.282  | 100.983 | 1.593 | -1.235 | 0.218 | 67.700 | 82.300  |
| MP97  | 331 | 26/11/2016 | 06:15 | magnetopause | in  | maybe not fully crossed | -15.166 | -98.883  | -1.974  | 56.883   | -82.293  | -1.974  | 100.059 | 1.591 | -0.966 | 0.226 | 67.200 | 81.400  |
| MP98  | 354 | 19/12/2016 | 01:50 | magnetopause | out |                         | -12.358 | -67.450  | -17.774 | -31.570  | -60.873  | -17.774 | 70.838  | 1.824 | -2.049 | 0.696 | nan    | nan     |
| MP99  | 354 | 19/12/2016 | 07:14 | magnetopause | in  |                         | -12.590 | -68.596  | -17.835 | 48.349   | 50.263   | -17.835 | 71.987  | 1.821 | 0.805  | 0.669 | 53.000 | 53.200  |
| MP100 | 354 | 19/12/2016 | 08:47 | magnetopause | out |                         | -12.653 | -68.910  | -17.851 | 69.328   | -10.110  | -17.851 | 72.300  | 1.820 | -0.145 | 0.662 | 53.100 | 53.500  |
| MP101 | 354 | 19/12/2016 | 14:12 | magnetopause | in  |                         | -12.880 | -70.025  | -17.905 | -64.648  | 29.833   | -17.905 | 73.417  | 1.817 | 2.709  | 0.637 | 53.600 | 54.600  |
| MP102 | 356 | 21/12/2016 | 08:48 | magnetopause | out | maybe not fully crossed | -14.549 | -78.039  | -18.135 | 53.524   | 58.625   | -18.135 | 81.428  | 1.795 | 0.831  | 0.483 | 57.100 | 62.000  |
| MP103 | 356 | 21/12/2016 | 15:37 | magnetopause | in  |                         | -14.795 | -79.191  | -18.144 | -76.944  | 23.869   | -18.144 | 82.579  | 1.792 | 2.841  | 0.464 | 57.600 | 63.000  |
| MP104 | 357 | 22/12/2016 | 06:05 | magnetopause | out |                         | -15.310 | -81.570  | -18.141 | 82.866   | -4.613   | -18.141 | 84.954  | 1.786 | -0.056 | 0.428 | 58.700 | 65.200  |
| MP105 | 357 | 22/12/2016 | 06:08 | magnetopause | in  |                         | -15.313 | -81.583  | -18.141 | 82.521   | -8.977   | -18.141 | 84.967  | 1.786 | -0.108 | 0.427 | 58.700 | 65.200  |
| MP106 | 357 | 22/12/2016 | 06:10 | magnetopause | out |                         | -15.313 | -81.583  | -18.141 | 82.521   | -8.977   | -18.141 | 84.967  | 1.786 | -0.108 | 0.427 | 58.700 | 65.200  |

# Supporting Information for “Effect of a magnetosphere compression on Jovian radio emissions: an in situ case study using Juno data”

|       |     |            |       |              |     |                         |         |          |         |          |          |         |         |       |        |       |        |        |
|-------|-----|------------|-------|--------------|-----|-------------------------|---------|----------|---------|----------|----------|---------|---------|-------|--------|-------|--------|--------|
| MP107 | 357 | 22/12/2016 | 09:09 | magnetopause | in  | maybe not fully crossed | -15.417 | -82.060  | -18.137 | -35.321  | -75.656  | -18.137 | 85.443  | 1.785 | -2.008 | 0.420 | 58.900 | 65.700 |
| MP108 | 366 | 31/12/2016 | 11:38 | magnetopause | out |                         | -21.038 | -104.823 | -15.515 | -54.345  | -92.071  | -15.514 | 108.033 | 1.715 | -2.104 | 0.189 | 69.600 | 85.800 |
| MP109 | 366 | 31/12/2016 | 18:00 | magnetopause | in  |                         | -21.149 | -105.184 | -15.388 | -105.748 | -18.120  | -15.388 | 108.387 | 1.713 | 0.170  | 0.187 | 69.800 | 86.000 |
| MP110 | 1   | 01/01/2017 | 04:26 | magnetopause | out |                         | -21.327 | -105.746 | -15.175 | 106.795  | -15.226  | -15.175 | 108.937 | 1.711 | -0.142 | 0.183 | 70.000 | 86.500 |
| MP111 | 1   | 01/01/2017 | 09:23 | magnetopause | in  |                         | -21.410 | -106.001 | -15.070 | -106.665 | 17.805   | -15.070 | 109.186 | 1.709 | 2.976  | 0.182 | 70.100 | 86.700 |
| MP112 | 1   | 01/01/2017 | 16:39 | magnetopause | out |                         | -21.527 | -106.354 | -14.917 | -4.642   | -108.412 | -14.917 | 109.532 | 1.707 | -1.614 | 0.179 | 70.300 | 87.000 |
| MP113 | 1   | 01/01/2017 | 22:09 | magnetopause | in  |                         | -21.613 | -106.610 | -14.798 | 40.662   | 100.894  | -14.798 | 109.781 | 1.706 | 1.188  | 0.178 | 70.400 | 87.200 |
| MP114 | 2   | 02/01/2017 | 13:47 | magnetopause | out |                         | -21.845 | -107.275 | -14.455 | -80.320  | -74.390  | -14.455 | 110.427 | 1.702 | -2.395 | 0.174 | 70.700 | 87.700 |
| MP115 | 4   | 04/01/2017 | 18:27 | magnetopause | in  |                         | -22.507 | -108.877 | -13.210 | -42.471  | 102.747  | -13.210 | 111.961 | 1.689 | 1.963  | 0.166 | 71.400 | 88.900 |
| MP116 | 11  | 11/01/2017 | 10:22 | magnetopause | out |                         | -23.304 | -107.812 | -8.763  | 34.280   | 104.840  | -8.763  | 110.650 | 1.650 | 1.255  | 0.180 | 70.200 | 86.900 |
| MP117 | 13  | 13/01/2017 | 03:18 | magnetopause | in  |                         | -23.191 | -106.085 | -7.490  | 98.637   | 45.415   | -7.490  | 108.848 | 1.640 | 0.431  | 0.195 | 69.200 | 85.000 |
| MP118 | 24  | 24/01/2017 | 20:01 | magnetopause | out |                         | -17.731 | -75.221  | 2.059   | 19.008   | -74.908  | 2.059   | 77.310  | 1.544 | -1.322 | 0.609 | 54.200 | 55.800 |
| MP119 | 24  | 24/01/2017 | 20:36 | magnetopause | in  |                         | -17.708 | -75.112  | 2.079   | -9.299   | -76.609  | 2.079   | 77.199  | 1.544 | -1.692 | 0.612 | 54.100 | 55.700 |
| MP120 | 24  | 24/01/2017 | 21:18 | magnetopause | out |                         | -17.678 | -74.973  | 2.105   | -43.213  | -63.766  | 2.105   | 77.057  | 1.543 | -2.166 | 0.614 | 54.100 | 55.500 |
| MP121 | 24  | 24/01/2017 | 22:38 | magnetopause | in  | maybe not fully crossed | -17.626 | -74.723  | 2.151   | -76.115  | -10.036  | 2.151   | 76.804  | 1.543 | -3.010 | 0.620 | 54.000 | 55.300 |
| MP122 | 25  | 25/01/2017 | 00:23 | magnetopause | out | maybe not fully crossed | -17.556 | -74.394  | 2.211   | -42.781  | 63.344   | 2.211   | 76.469  | 1.542 | 2.165  | 0.627 | 53.800 | 55.000 |
| MP123 | 25  | 25/01/2017 | 17:53 | magnetopause | in  |                         | -16.826 | -70.971  | 2.811   | -63.629  | -35.655  | 2.811   | 72.992  | 1.532 | -2.631 | 0.703 | nan    | nan    |
| MP124 | 42  | 11/02/2017 | 01:42 | magnetopause | out | maybe not fully crossed | -18.377 | -71.730  | -19.226 | 56.907   | 47.376   | -19.226 | 76.501  | 1.825 | 0.694  | 0.657 | 53.200 | 53.700 |
| MP125 | 42  | 11/02/2017 | 19:08 | magnetopause | in  |                         | -19.279 | -74.919  | -19.363 | -44.379  | 63.365   | -19.363 | 79.746  | 1.816 | 2.182  | 0.591 | 54.500 | 56.600 |
| MP126 | 50  | 19/02/2017 | 04:33 | magnetopause | out |                         | -26.188 | -97.532  | -18.467 | -99.343  | 18.145   | -18.467 | 102.661 | 1.752 | 2.961  | 0.279 | 64.300 | 76.200 |
| MP127 | 50  | 19/02/2017 | 04:50 | magnetopause | in  |                         | -26.195 | -97.553  | -18.463 | -95.263  | 33.583   | -18.463 | 102.683 | 1.752 | 2.803  | 0.279 | 64.300 | 76.200 |
| MP128 | 50  | 19/02/2017 | 06:01 | magnetopause | out |                         | -26.229 | -97.653  | -18.447 | -47.879  | 89.060   | -18.447 | 102.783 | 1.751 | 2.064  | 0.278 | 64.400 | 76.300 |
| MP129 | 50  | 19/02/2017 | 10:15 | magnetopause | in  | maybe not fully crossed | -26.352 | -98.013  | -18.388 | 82.219   | -59.507  | -18.388 | 103.146 | 1.750 | -0.626 | 0.275 | 64.500 | 76.600 |
| MP130 | 50  | 19/02/2017 | 10:50 | magnetopause | out | maybe not fully crossed | -26.368 | -98.062  | -18.379 | 55.225   | -85.216  | -18.380 | 103.195 | 1.750 | -0.996 | 0.274 | 64.500 | 76.600 |
| MP131 | 53  | 22/02/2017 | 04:21 | magnetopause | in  | maybe not fully crossed | -28.035 | -102.697 | -17.298 | 5.394    | 106.318  | -17.298 | 107.851 | 1.732 | 1.520  | 0.236 | 66.600 | 80.400 |
| MP132 | 63  | 04/03/2017 | 20:49 | magnetopause | out | maybe not fully crossed | -30.670 | -106.103 | -10.873 | -88.433  | 66.168   | -10.873 | 110.981 | 1.669 | 2.499  | 0.223 | 67.400 | 81.800 |
| MP133 | 64  | 05/03/2017 | 08:24 | magnetopause | in  |                         | -30.637 | -105.723 | -10.518 | 13.341   | 109.262  | -10.518 | 110.575 | 1.666 | 1.449  | 0.226 | 67.100 | 81.400 |
| MP134 | 67  | 08/03/2017 | 15:17 | magnetopause | out |                         | -30.031 | -101.863 | -7.977  | -24.885  | 103.241  | -7.977  | 106.497 | 1.646 | 1.807  | 0.265 | 65.000 | 77.500 |
| MP135 | 68  | 09/03/2017 | 07:05 | magnetopause | in  | maybe not fully crossed | -29.823 | -100.810 | -7.443  | -37.269  | -98.301  | -7.443  | 105.392 | 1.641 | -1.933 | 0.276 | 64.400 | 76.400 |
| MP136 | 68  | 09/03/2017 | 09:58 | magnetopause | out | maybe not fully crossed | -29.781 | -100.606 | -7.344  | -84.278  | 62.495   | -7.344  | 105.178 | 1.641 | 2.504  | 0.279 | 64.300 | 76.200 |
| MP137 | 68  | 09/03/2017 | 13:53 | magnetopause | in  | maybe not fully crossed | -29.724 | -100.326 | -7.211  | 104.606  | 2.509    | -7.211  | 104.884 | 1.640 | 0.024  | 0.282 | 64.200 | 76.000 |
| MP138 | 68  | 09/03/2017 | 14:57 | magnetopause | out |                         | -29.709 | -100.253 | -7.176  | 85.759   | -59.823  | -7.176  | 104.809 | 1.639 | -0.609 | 0.282 | 64.200 | 75.900 |
| MP139 | 68  | 09/03/2017 | 15:21 | magnetopause | in  |                         | -29.702 | -100.223 | -7.162  | 67.175   | -80.091  | -7.162  | 104.777 | 1.639 | -0.873 | 0.283 | 64.100 | 75.900 |
| MP140 | 69  | 10/03/2017 | 00:50 | magnetopause | out |                         | -29.554 | -99.515  | -6.836  | 85.448   | -58.951  | -6.836  | 104.035 | 1.637 | -0.604 | 0.290 | 63.800 | 75.200 |
| MP141 | 69  | 10/03/2017 | 08:53 | magnetopause | in  |                         | -29.419 | -98.884  | -6.557  | 87.305   | 54.967   | -6.557  | 103.376 | 1.634 | 0.562  | 0.297 | 63.500 | 74.600 |
| MP142 | 71  | 12/03/2017 | 13:14 | magnetopause | out | maybe not fully crossed | -28.332 | -94.152  | -4.709  | 39.877   | -89.873  | -4.709  | 98.435  | 1.619 | -1.153 | 0.354 | 61.100 | 70.100 |
| MP143 | 71  | 12/03/2017 | 19:48 | magnetopause | in  |                         | -28.169 | -93.473  | -4.472  | 55.811   | 80.099   | -4.472  | 97.728  | 1.617 | 0.962  | 0.363 | 60.800 | 69.500 |
| MP144 | 98  | 08/04/2017 | 15:02 | magnetopause | out |                         | -28.193 | -84.014  | -20.863 | -52.364  | 71.493   | -20.863 | 91.041  | 1.802 | 2.203  | 0.485 | 57.100 | 61.900 |
| MP145 | 100 | 10/04/2017 | 00:05 | magnetopause | in  |                         | -29.761 | -88.082  | -20.754 | 92.431   | 10.035   | -20.753 | 95.263  | 1.790 | 0.108  | 0.426 | 58.700 | 65.300 |
| MP146 | 101 | 11/04/2017 | 10:26 | magnetopause | out |                         | -31.226 | -91.770  | -20.515 | -90.600  | -34.473  | -20.515 | 99.084  | 1.779 | -2.778 | 0.379 | 60.200 | 68.300 |
| MP147 | 102 | 12/04/2017 | 03:49 | magnetopause | in  |                         | -31.907 | -93.445  | -20.351 | 32.281   | -93.316  | -20.351 | 100.817 | 1.774 | -1.238 | 0.360 | 60.900 | 69.700 |
| MP148 | 102 | 12/04/2017 | 21:17 | magnetopause | out |                         | -32.548 | -94.994  | -20.159 | 95.856   | 29.917   | -20.159 | 102.419 | 1.769 | 0.303  | 0.343 | 61.600 | 71.000 |
| MP149 | 103 | 13/04/2017 | 13:39 | magnetopause | in  | maybe not fully crossed | -33.117 | -96.343  | -19.955 | -80.123  | 62.921   | -19.955 | 103.812 | 1.764 | 2.476  | 0.329 | 62.100 | 72.000 |
| MP150 | 109 | 19/04/2017 | 16:18 | magnetopause | out |                         | -36.773 | -103.963 | -17.274 | -82.120  | -73.598  | -17.274 | 111.619 | 1.726 | -2.411 | 0.262 | 65.100 | 77.700 |
| MP151 | 110 | 20/04/2017 | 08:26 | magnetopause | in  |                         | -37.019 | -104.342 | -16.899 | 110.675  | -2.931   | -16.899 | 111.996 | 1.722 | -0.026 | 0.260 | 65.300 | 78.000 |
| MP152 | 125 | 05/05/2017 | 13:14 | magnetopause | out |                         | -33.872 | -89.079  | -5.282  | 8.323    | 94.938   | -5.283  | 95.448  | 1.626 | 1.483  | 0.473 | 57.400 | 62.600 |
| MP153 | 126 | 06/05/2017 | 18:12 | magnetopause | in  | maybe not fully crossed | -32.756 | -85.667  | -4.161  | -40.350  | 82.364   | -4.161  | 91.811  | 1.616 | 2.026  | 0.529 | 55.900 | 59.600 |
| MP154 | 126 | 06/05/2017 | 21:04 | magnetopause | out | maybe not fully crossed | -32.635 | -85.301  | -4.046  | 89.857   | 16.337   | -4.046  | 91.420  | 1.615 | 0.180  | 0.536 | 55.800 | 59.200 |
| MP155 | 126 | 06/05/2017 | 23:57 | magnetopause | in  | maybe not fully crossed | -32.515 | -84.941  | -3.935  | -3.918   | -90.867  | -3.935  | 91.036  | 1.614 | -1.614 | 0.542 | 55.600 | 58.900 |
| MP156 | 151 | 31/05/2017 | 13:02 | magnetopause | out |                         | -33.709 | -81.687  | -22.278 | -68.169  | 56.231   | -22.278 | 91.134  | 1.818 | 2.452  | 0.574 | 54.900 | 57.400 |
| MP157 | 151 | 31/05/2017 | 21:38 | magnetopause | in  |                         | -34.211 | -82.768  | -22.280 | -89.049  | -9.541   | -22.280 | 92.289  | 1.815 | -3.035 | 0.555 | 55.300 | 58.300 |
| MP158 | 152 | 01/06/2017 | 18:17 | magnetopause | out | maybe not fully crossed | -35.347 | -85.193  | -22.246 | -86.392  | 32.304   | -22.246 | 94.879  | 1.807 | 2.784  | 0.516 | 56.300 | 60.200 |
| MP159 | 153 | 02/06/2017 | 01:25 | magnetopause | in  | maybe not fully crossed | -35.725 | -85.991  | -22.222 | -16.902  | -91.570  | -22.222 | 95.732  | 1.805 | -1.753 | 0.504 | 56.600 | 60.900 |
| MP160 | 153 | 02/06/2017 | 20:46 | magnetopause | out |                         | -36.703 | -88.030  | -22.129 | 13.712   | -94.385  | -22.129 | 97.909  | 1.799 | -1.427 | 0.474 | 57.300 | 62.500 |
| MP161 | 153 | 02/06/2017 | 23:46 | magnetopause | in  |                         | -36.849 | -88.333  | -22.111 | -94.091  | 17.529   | -22.111 | 98.231  | 1.798 | 2.957  | 0.470 | 57.500 | 62.700 |
| MP162 | 157 | 06/06/2017 | 00:18 | magnetopause | out |                         | -39.952 | -94.528  | -21.408 | 56.431   | 85.717   | -21.408 | 104.834 | 1.776 | 0.989  | 0.391 | 59.800 | 67.500 |
| MP163 | 157 | 06/06/2017 | 00:30 | magnetopause | in  |                         | -39.959 | -94.540  | -21.406 | 65.153   | 79.307   | -21.406 | 104.846 | 1.776 | 0.883  | 0.391 | 59.800 | 67.500 |
| MP164 | 167 | 16/06/2017 | 08:18 | magnetopause | out |                         | -44.844 | -101.628 | -16.071 | 53.878   | 97.141   | -16.071 | 112.238 | 1.714 | 1.064  | 0.332 | 62.000 | 71.800 |

# Supporting Information for “Effect of a magnetosphere compression on Jovian radio emissions: an in situ case study using Juno data”

|       |     |            |       |              |     |                         |         |          |         |          |          |         |         |       |        |       |        |        |
|-------|-----|------------|-------|--------------|-----|-------------------------|---------|----------|---------|----------|----------|---------|---------|-------|--------|-------|--------|--------|
| MP165 | 167 | 16/06/2017 | 09:58 | magnetopause | in  |                         | -44.848 | -101.607 | -16.023 | 111.060  | 1.029    | -16.023 | 112.215 | 1.714 | 0.009  | 0.332 | 62.000 | 71.800 |
| MP166 | 167 | 16/06/2017 | 10:46 | magnetopause | out |                         | -44.849 | -101.598 | -16.001 | 99.237   | -49.854  | -16.001 | 112.203 | 1.714 | -0.466 | 0.332 | 62.000 | 71.800 |
| MP167 | 168 | 17/06/2017 | 14:12 | magnetopause | in  |                         | -44.851 | -101.123 | -15.189 | 57.229   | 94.669   | -15.189 | 111.661 | 1.707 | 1.027  | 0.340 | 61.700 | 71.200 |
| MP168 | 169 | 18/06/2017 | 09:02 | magnetopause | out |                         | -44.788 | -100.655 | -14.609 | -10.957  | 109.623  | -14.609 | 111.134 | 1.703 | 1.670  | 0.347 | 61.400 | 70.600 |
| MP169 | 169 | 18/06/2017 | 23:42 | magnetopause | in  |                         | -44.703 | -100.210 | -14.146 | 25.999   | -106.604 | -14.146 | 110.637 | 1.699 | -1.332 | 0.354 | 61.200 | 70.200 |
| MP170 | 170 | 19/06/2017 | 01:44 | magnetopause | out | maybe not fully crossed | -44.688 | -100.141 | -14.079 | -96.700  | -51.714  | -14.079 | 110.559 | 1.698 | -2.651 | 0.355 | 61.100 | 70.100 |
| MP171 | 170 | 19/06/2017 | 03:35 | magnetopause | in  |                         | -44.675 | -100.079 | -14.020 | -85.935  | 68.020   | -14.020 | 110.491 | 1.698 | 2.472  | 0.355 | 61.100 | 70.000 |
| MP172 | 178 | 27/06/2017 | 21:27 | magnetopause | out |                         | -39.372 | -85.043  | -6.337  | -0.601   | 93.713   | -6.337  | 93.929  | 1.638 | 1.577  | 0.597 | 54.400 | 56.300 |
| MP173 | 179 | 28/06/2017 | 12:58 | magnetopause | in  | maybe not fully crossed | -38.635 | -83.220  | -5.698  | -38.614  | -83.230  | -5.698  | 91.928  | 1.633 | -2.005 | 0.633 | 53.700 | 54.700 |
| MP174 | 179 | 28/06/2017 | 14:48 | magnetopause | out | maybe not fully crossed | -38.545 | -82.998  | -5.623  | -91.485  | 2.218    | -5.623  | 91.684  | 1.632 | 3.117  | 0.637 | 53.600 | 54.500 |
| MP175 | 179 | 28/06/2017 | 18:10 | magnetopause | in  |                         | -38.378 | -82.590  | -5.485  | 48.664   | 76.980   | -5.485  | 91.237  | 1.631 | 1.007  | 0.645 | 53.500 | 54.200 |
| MP176 | 179 | 28/06/2017 | 21:11 | magnetopause | out |                         | -38.226 | -82.219  | -5.361  | 56.915   | -70.583  | -5.361  | 90.829  | 1.630 | -0.892 | 0.653 | 53.300 | 53.900 |
| MP177 | 180 | 29/06/2017 | 01:58 | magnetopause | in  | maybe not fully crossed | -37.977 | -81.611  | -5.160  | -62.031  | 65.228   | -5.160  | 90.162  | 1.628 | 2.331  | 0.666 | 53.100 | 53.400 |
| MP178 | 180 | 29/06/2017 | 02:18 | magnetopause | out | maybe not fully crossed | -37.959 | -81.568  | -5.146  | -46.968  | 76.735   | -5.146  | 90.116  | 1.628 | 2.120  | 0.666 | 53.100 | 53.300 |
| MP179 | 180 | 29/06/2017 | 02:40 | magnetopause | in  | maybe not fully crossed | -37.942 | -81.526  | -5.132  | -29.837  | 84.828   | -5.132  | 90.069  | 1.628 | 1.909  | 0.667 | 53.000 | 53.300 |
| MP180 | 180 | 29/06/2017 | 02:53 | magnetopause | out | maybe not fully crossed | -37.929 | -81.494  | -5.121  | -16.088  | 88.437   | -5.122  | 90.034  | 1.628 | 1.751  | 0.668 | 53.000 | 53.300 |
| MP181 | 180 | 29/06/2017 | 02:58 | magnetopause | in  | maybe not fully crossed | -37.925 | -81.484  | -5.118  | -11.401  | 89.151   | -5.118  | 90.022  | 1.628 | 1.698  | 0.668 | 53.000 | 53.200 |
| MP182 | 180 | 29/06/2017 | 03:43 | magnetopause | out | maybe not fully crossed | -37.885 | -81.388  | -5.087  | 30.582   | 84.404   | -5.087  | 89.917  | 1.627 | 1.223  | 0.670 | 53.000 | 53.200 |
| MP183 | 180 | 29/06/2017 | 04:05 | magnetopause | in  | maybe not fully crossed | -37.868 | -81.345  | -5.073  | 47.559   | 76.086   | -5.073  | 89.871  | 1.627 | 1.012  | 0.671 | 53.000 | 53.100 |
| MP184 | 180 | 29/06/2017 | 04:17 | magnetopause | out | maybe not fully crossed | -37.859 | -81.324  | -5.066  | 55.294   | 70.636   | -5.066  | 89.847  | 1.627 | 0.907  | 0.672 | 53.000 | 53.100 |
| MP185 | 180 | 29/06/2017 | 05:14 | magnetopause | in  | maybe not fully crossed | -37.806 | -81.195  | -5.024  | 86.235   | 24.196   | -5.024  | 89.706  | 1.627 | 0.274  | 0.674 | 52.900 | 53.000 |
| MP186 | 180 | 29/06/2017 | 05:41 | magnetopause | out |                         | -37.784 | -81.142  | -5.007  | 89.503   | 0.874    | -5.007  | 89.648  | 1.627 | 0.010  | 0.675 | 52.900 | 53.000 |
| MP187 | 180 | 29/06/2017 | 05:44 | magnetopause | in  |                         | -37.779 | -81.131  | -5.003  | 89.413   | -3.847   | -5.003  | 89.636  | 1.627 | -0.043 | 0.676 | nan    | nan    |
| MP188 | 180 | 29/06/2017 | 07:46 | magnetopause | out | maybe not fully crossed | -37.673 | -80.872  | -4.920  | 23.076   | -86.180  | -4.920  | 89.352  | 1.626 | -1.309 | 0.681 | nan    | nan    |
| MP189 | 180 | 29/06/2017 | 09:31 | magnetopause | in  | maybe not fully crossed | -37.578 | -80.645  | -4.846  | -66.622  | -58.968  | -4.846  | 89.102  | 1.625 | -2.417 | 0.686 | nan    | nan    |
| MP190 | 220 | 08/08/2017 | 08:28 | magnetopause | out |                         | -51.510 | -98.051  | -17.746 | 110.567  | -6.494   | -17.746 | 112.170 | 1.730 | -0.059 | 0.417 | 59.000 | 65.900 |
| MP191 | 220 | 08/08/2017 | 08:40 | magnetopause | in  |                         | -51.510 | -98.049  | -17.741 | 109.267  | -18.102  | -17.741 | 112.168 | 1.730 | -0.164 | 0.417 | 59.000 | 65.900 |
| MP192 | 225 | 13/08/2017 | 00:52 | magnetopause | out |                         | -50.588 | -94.565  | -14.122 | -50.397  | -94.666  | -14.122 | 108.171 | 1.702 | -2.060 | 0.478 | 57.200 | 62.300 |
| MP193 | 225 | 13/08/2017 | 03:43 | magnetopause | in  |                         | -50.534 | -94.420  | -14.019 | -77.262  | 74.157   | -14.019 | 108.006 | 1.701 | 2.377  | 0.481 | 57.200 | 62.100 |
| MP194 | 257 | 14/09/2017 | 23:21 | magnetopause | out | maybe not fully crossed | -45.232 | -77.930  | -25.155 | 88.947   | 14.408   | -25.155 | 93.551  | 1.843 | 0.161  | 0.766 | nan    | nan    |
| MP195 | 258 | 15/09/2017 | 18:42 | magnetopause | in  | maybe not fully crossed | -46.564 | -79.961  | -25.179 | 81.765   | 43.319   | -25.179 | 95.896  | 1.836 | 0.487  | 0.724 | nan    | nan    |
| MP196 | 274 | 01/10/2017 | 05:48 | magnetopause | out |                         | -57.857 | -93.646  | -18.705 | -47.369  | -99.363  | -18.705 | 111.655 | 1.739 | -2.016 | 0.532 | 55.900 | 59.400 |
| MP197 | 275 | 02/10/2017 | 18:29 | magnetopause | in  |                         | -57.588 | -92.681  | -17.528 | 108.613  | -10.466  | -17.528 | 110.515 | 1.730 | -0.096 | 0.553 | 55.400 | 58.400 |
| MP198 | 275 | 02/10/2017 | 18:52 | magnetopause | out |                         | -57.585 | -92.671  | -17.517 | 104.001  | -32.981  | -17.517 | 110.502 | 1.730 | -0.307 | 0.553 | 55.400 | 58.400 |
| MP199 | 275 | 02/10/2017 | 22:39 | magnetopause | in  |                         | -57.541 | -92.546  | -17.389 | -100.045 | -43.206  | -17.389 | 110.354 | 1.729 | -2.734 | 0.556 | 55.300 | 58.200 |
| MP200 | 276 | 03/10/2017 | 01:54 | magnetopause | out |                         | -57.503 | -92.436  | -17.280 | 8.598    | 108.522  | -17.280 | 110.225 | 1.728 | 1.492  | 0.558 | 55.300 | 58.100 |
| MP201 | 276 | 03/10/2017 | 08:56 | magnetopause | in  |                         | -57.412 | -92.190  | -17.043 | -106.403 | -21.759  | -17.043 | 109.934 | 1.726 | -2.940 | 0.563 | 55.100 | 57.900 |
| MP202 | 314 | 10/11/2017 | 11:18 | magnetopause | out | maybe not fully crossed | -56.039 | -82.163  | -26.521 | -80.503  | 58.398   | -26.521 | 102.930 | 1.831 | 2.514  | 0.749 | nan    | nan    |
| MP203 | 314 | 10/11/2017 | 12:56 | magnetopause | in  | maybe not fully crossed | -56.130 | -82.275  | -26.511 | 5.891    | 99.424   | -26.511 | 103.066 | 1.831 | 1.512  | 0.747 | nan    | nan    |
| MP204 | 6   | 06/01/2018 | 08:43 | magnetopause | out | maybe not fully crossed | -65.768 | -82.730  | -27.038 | 48.536   | -93.883  | -27.038 | 109.090 | 1.821 | -1.094 | 0.821 | nan    | nan    |
| MP205 | 6   | 06/01/2018 | 11:19 | magnetopause | in  | maybe not fully crossed | -65.872 | -82.827  | -26.999 | -96.953  | -42.421  | -26.999 | 109.217 | 1.821 | -2.729 | 0.820 | nan    | nan    |
| MP206 | 167 | 16/06/2018 | 13:24 | magnetopause | out | maybe not fully crossed | -82.206 | -69.083  | -30.792 | 104.771  | 23.524   | -30.792 | 111.707 | 1.850 | 0.221  | 1.546 | nan    | nan    |
| MP207 | 167 | 16/06/2018 | 13:35 | magnetopause | in  | maybe not fully crossed | -82.211 | -69.085  | -30.789 | 106.671  | 12.359   | -30.789 | 111.711 | 1.850 | 0.115  | 1.546 | nan    | nan    |
| MP208 | 167 | 16/06/2018 | 13:51 | magnetopause | out | maybe not fully crossed | -82.219 | -69.089  | -30.784 | 107.294  | -4.609   | -30.784 | 111.718 | 1.850 | -0.043 | 1.546 | nan    | nan    |
| MP209 | 167 | 16/06/2018 | 14:03 | magnetopause | in  | maybe not fully crossed | -82.227 | -69.092  | -30.780 | 105.235  | -21.464  | -30.780 | 111.725 | 1.850 | -0.201 | 1.546 | nan    | nan    |
| MP210 | 167 | 16/06/2018 | 14:28 | magnetopause | out | maybe not fully crossed | -82.240 | -69.098  | -30.772 | 96.010   | -48.167  | -30.772 | 111.736 | 1.850 | -0.465 | 1.546 | nan    | nan    |
| MP211 | 167 | 16/06/2018 | 15:13 | magnetopause | in  | maybe not fully crossed | -82.263 | -69.108  | -30.758 | 63.382   | -86.752  | -30.758 | 111.755 | 1.850 | -0.940 | 1.546 | nan    | nan    |
| MP212 | 167 | 16/06/2018 | 16:14 | magnetopause | out | maybe not fully crossed | -82.294 | -69.121  | -30.739 | -0.229   | -107.471 | -30.739 | 111.781 | 1.849 | -1.573 | 1.546 | nan    | nan    |
| MP213 | 167 | 16/06/2018 | 17:09 | magnetopause | in  | maybe not fully crossed | -82.322 | -69.133  | -30.722 | -59.136  | -89.774  | -30.722 | 111.804 | 1.849 | -2.153 | 1.546 | nan    | nan    |
| MP214 | 216 | 04/08/2018 | 06:30 | magnetopause | out | maybe not fully crossed | -81.227 | -60.943  | -33.601 | 3.763    | 101.478  | -33.601 | 106.963 | 1.890 | 1.534  | 2.028 | nan    | nan    |
| MP215 | 216 | 04/08/2018 | 08:51 | magnetopause | in  | maybe not fully crossed | -81.369 | -61.021  | -33.585 | 101.546  | 5.740    | -33.585 | 107.110 | 1.890 | 0.056  | 2.025 | nan    | nan    |
| MP216 | 359 | 25/12/2021 | 19:45 | magnetopause | out |                         | -50.810 | 67.232   | -47.743 | 50.583   | -67.403  | -47.743 | 96.857  | 2.086 | -0.927 | 1.022 | nan    | nan    |
| MP217 | 360 | 26/12/2021 | 12:10 | magnetopause | in  |                         | -50.377 | 66.959   | -46.894 | 26.790   | 79.395   | -46.894 | 96.022  | 2.081 | 1.245  | 1.043 | nan    | nan    |
| MP218 | 47  | 16/02/2022 | 06:25 | magnetopause | out | maybe not fully crossed | -35.828 | 57.448   | -32.540 | 66.295   | 13.742   | -32.540 | 75.118  | 2.019 | 0.204  | 1.572 | nan    | nan    |
| MP219 | 47  | 16/02/2022 | 11:15 | magnetopause | in  |                         | -35.436 | 56.919   | -32.012 | -64.332  | -18.893  | -32.012 | 74.299  | 2.016 | -2.856 | 1.610 | nan    | nan    |
| MP220 | 78  | 19/03/2022 | 08:17 | magnetopause | out |                         | -42.546 | 71.335   | -53.552 | 63.877   | -53.090  | -53.552 | 98.826  | 2.143 | -0.693 | 0.694 | nan    | nan    |
| MP221 | 78  | 19/03/2022 | 22:59 | magnetopause | in  |                         | -42.482 | 71.530   | -53.111 | -68.316  | 47.478   | -53.111 | 98.702  | 2.139 | 2.534  | 0.695 | nan    | nan    |
| MP222 | 359 | 25/12/2022 | 20:11 | magnetopause | out | maybe not fully crossed | -9.565  | 56.417   | -54.489 | 17.767   | 54.390   | -54.492 | 79.015  | 2.332 | 1.255  | 0.629 | 53.800 | 54.900 |

# Supporting Information for “Effect of a magnetosphere compression on Jovian radio emissions: an in situ case study using Juno data”

|       |     |            |       |              |     |                         |         |        |         |         |         |         |        |       |        |       |        |        |
|-------|-----|------------|-------|--------------|-----|-------------------------|---------|--------|---------|---------|---------|---------|--------|-------|--------|-------|--------|--------|
| MP223 | 359 | 25/12/2022 | 20:28 | magnetopause | in  | maybe not fully crossed | -9.568  | 56.454 | -54.507 | 28.785  | 49.493  | -54.510 | 79.054 | 2.332 | 1.044  | 0.628 | 53.800 | 55.000 |
| MP224 | 360 | 26/12/2022 | 06:23 | magnetopause | out | maybe not fully crossed | -9.649  | 57.531 | -55.018 | 29.116  | 50.545  | -55.021 | 80.186 | 2.327 | 1.048  | 0.590 | 54.600 | 56.600 |
| MP225 | 359 | 25/12/2022 | 12:13 | magnetopause | in  |                         | -9.493  | 55.519 | -54.045 | 56.315  | -0.869  | -54.048 | 78.060 | 2.336 | -0.015 | 0.662 | 53.100 | 53.500 |
| MP226 | 47  | 16/02/2022 | 07:17 | magnetopause | out | maybe not fully crossed | -35.761 | 57.357 | -32.450 | 64.092  | -21.471 | -32.450 | 74.978 | 2.018 | -0.323 | 1.579 | nan    | nan    |
| MP227 | 47  | 16/02/2022 | 11:15 | magnetopause | in  |                         | -35.436 | 56.919 | -32.012 | -64.332 | -18.893 | -32.012 | 74.299 | 2.016 | -2.856 | 1.610 | nan    | nan    |
| MP228 | 78  | 19/03/2022 | 08:20 | magnetopause | out | maybe not fully crossed | -42.546 | 71.336 | -53.550 | 60.989  | -56.385 | -53.550 | 98.826 | 2.143 | -0.746 | 0.694 | nan    | nan    |
| MP229 | 78  | 19/03/2022 | 22:59 | magnetopause | in  | maybe not fully crossed | -42.482 | 71.530 | -53.111 | -68.316 | 47.478  | -53.111 | 98.702 | 2.139 | 2.534  | 0.695 | nan    | nan    |
| MP230 | 128 | 08/05/2022 | 12:52 | magnetopause | out |                         | -34.772 | 70.862 | -46.883 | -78.328 | -9.756  | -46.883 | 91.807 | 2.107 | -3.018 | 0.716 | nan    | nan    |
| MP231 | 128 | 08/05/2022 | 15:42 | magnetopause | in  |                         | -34.679 | 70.737 | -46.685 | 7.799   | 78.393  | -46.685 | 91.574 | 2.106 | 1.472  | 0.721 | nan    | nan    |
| MP232 | 158 | 07/06/2022 | 21:52 | magnetopause | out |                         | -31.399 | 67.784 | -56.902 | 67.114  | 32.806  | -56.902 | 93.906 | 2.222 | 0.455  | 0.606 | 54.200 | 55.900 |
| MP233 | 159 | 08/06/2022 | 06:56 | magnetopause | in  |                         | -31.582 | 68.396 | -57.022 | 41.535  | 62.851  | -57.022 | 94.482 | 2.219 | 0.987  | 0.591 | 54.600 | 56.600 |
| MP234 | 159 | 08/06/2022 | 11:12 | magnetopause | out |                         | -31.663 | 68.672 | -57.069 | -10.043 | -74.950 | -57.069 | 94.737 | 2.217 | -1.704 | 0.584 | 54.700 | 56.900 |
| MP235 | 159 | 08/06/2022 | 11:28 | magnetopause | in  |                         | -31.669 | 68.693 | -57.072 | -25.528 | -71.203 | -57.072 | 94.757 | 2.217 | -1.915 | 0.584 | 54.700 | 56.900 |
| MP236 | 159 | 08/06/2022 | 11:40 | magnetopause | out |                         | -31.672 | 68.704 | -57.074 | -32.891 | -68.128 | -57.074 | 94.767 | 2.217 | -2.021 | 0.584 | 54.700 | 56.900 |
| MP237 | 159 | 08/06/2022 | 16:33 | magnetopause | in  | maybe not fully crossed | -31.761 | 69.013 | -57.121 | 31.054  | 69.334  | -57.121 | 95.050 | 2.215 | 1.150  | 0.577 | 54.900 | 57.300 |
| MP238 | 160 | 09/06/2022 | 00:54 | magnetopause | out |                         | -31.902 | 69.519 | -57.184 | -42.298 | 63.730  | -57.184 | 95.502 | 2.213 | 2.157  | 0.565 | 55.100 | 57.800 |
| MP239 | 160 | 09/06/2022 | 10:12 | magnetopause | in  |                         | -32.044 | 70.051 | -57.231 | -65.341 | 40.798  | -57.231 | 95.965 | 2.210 | 2.583  | 0.554 | 55.400 | 58.300 |
| MP240 | 160 | 09/06/2022 | 12:45 | magnetopause | out |                         | -32.081 | 70.194 | -57.239 | 45.029  | 62.680  | -57.239 | 96.087 | 2.209 | 0.948  | 0.551 | 55.400 | 58.500 |
| MP241 | 161 | 10/06/2022 | 15:44 | magnetopause | in  |                         | -32.401 | 71.552 | -57.213 | -71.104 | 33.373  | -57.213 | 97.174 | 2.200 | 2.703  | 0.525 | 56.000 | 59.800 |
| MP242 | 168 | 17/06/2022 | 13:21 | magnetopause | out |                         | -31.832 | 74.302 | -52.727 | -2.511  | -80.794 | -52.727 | 96.510 | 2.149 | -1.602 | 0.520 | 56.200 | 60.000 |
| MP243 | 169 | 18/06/2022 | 17:45 | magnetopause | in  |                         | -31.302 | 73.778 | -51.230 | 58.983  | -54.260 | -51.230 | 95.119 | 2.140 | -0.744 | 0.545 | 55.600 | 58.800 |

Supporting Information for “Effect of a magnetosphere compression on Jovian radio emissions: an in situ case study using Juno data”

**Table S1 – List of Magnetopause boundary crossings from Juno/Waves and Juno/MAG measurements**

All this information is also available directly in the file:  
*boundary\_crossings\_characteristics\_list.csv* (File F1).

*Table S 2: List of bow shock crossings, as measured by Juno/Waves and Juno/MAG. For each crossing, number of the crossing (MP#), day of the year (DOY), date (day/month/year format) and time (hours:minutes format) are indicated, as well as the boundary crossed (bow shock in this case), the direction of the crossing (in: from the magnetosheath to the solar wind; out: from the solar wind to the magnetosheath). Position of the crossings are given in the Cartesian Jupiter-Heliospheric (JH) and the International Astronomical Union (IAU) coordinate systems, and IAU spherical coordinates system. Finally, the dynamic pressure of the solar wind, and the standoff distance of the magnetopause and the bow shock, derived from the model of Joy et al. (2002), are given in the last three columns. Note that the list of crossings up to 2016-11-26 was provided by Hospodarsky et al. (2017).*

## Supporting Information for “Effect of a magnetosphere compression on Jovian radio emissions: an in situ case study using Juno data”

- (1) JSS coordinate system: this coordinate system is defined such that X points towards the Sun, the Z axis is along the Jovian spin axis, positive in the direction of angular momentum, and Y completes the righthanded set (positive towards dusk).  
 (2) IAU coordinate system: this coordinate system is defined such that Z-axis is along the Jovian spin axis, X-axis is defined by 0° latitude on the System III longitude  $\lambda_{III} = 0^\circ$  (prime meridian). The Y-axis completes the orthogonal right-handed system.  
 (3) Values determined using the Joy et al. (2002)'s model  
 Note: the nan values in the 'standoff distance' columns are given when the bow shock standoff distance calculated from the Joy et al. (2002) model is smaller than that of the magnetopause (non-physical).

| #    | Day of Year | Date<br>(day/month/year) | Time<br>(HH:MM) | Boundary  | in/out | Notes | x<br>(JSS <sup>1</sup> ) | y<br>(JSS <sup>1</sup> ) | z<br>(JSS <sup>1</sup> ) | x<br>(IAU <sup>2</sup> ) | y<br>(IAU <sup>2</sup> ) | z<br>(IAU <sup>2</sup> ) | r<br>(IAU <sup>2</sup> ) | $\theta$<br>(IAU <sup>2</sup> ) | $\phi$<br>(IAU <sup>2</sup> ) | Dynamic<br>Pressure <sup>3</sup><br>(nPa) | Magnetopause<br>Standoff<br>Distance <sup>3</sup><br>(Jovian radius) | Bow Shock<br>Standoff<br>Distance <sup>3</sup><br>(Jovian radius) |
|------|-------------|--------------------------|-----------------|-----------|--------|-------|--------------------------|--------------------------|--------------------------|--------------------------|--------------------------|--------------------------|--------------------------|---------------------------------|-------------------------------|-------------------------------------------|----------------------------------------------------------------------|-------------------------------------------------------------------|
| BS1  | 176         | 24/06/2016               | 08:16           | bow shock | in     |       | 6.723                    | -124.901                 | 27.698                   | -120.972                 | 31.800                   | 27.698                   | 128.112                  | 1.353                           | 2.885                         | 0.212                                     | 68.000                                                               | 83.000                                                            |
| BS2  | 199         | 17/07/2016               | 15:33           | bow shock | out    |       | 1.982                    | -91.079                  | -13.748                  | 72.872                   | 54.671                   | -13.748                  | 92.132                   | 1.721                           | 0.644                         | 0.617                                     | 54.000                                                               | 55.400                                                            |
| BS3  | 200         | 18/07/2016               | 01:22           | bow shock | in     |       | 1.961                    | -92.393                  | -13.618                  | 67.341                   | 63.289                   | -13.618                  | 93.412                   | 1.717                           | 0.754                         | 0.597                                     | 54.400                                                               | 56.300                                                            |
| BS4  | 200         | 18/07/2016               | 02:21           | bow shock | out    |       | 1.959                    | -92.525                  | -13.605                  | 91.866                   | 11.200                   | -13.604                  | 93.541                   | 1.717                           | 0.121                         | 0.595                                     | 54.500                                                               | 56.400                                                            |
| BS5  | 200         | 18/07/2016               | 21:18           | bow shock | in     |       | 1.911                    | -94.939                  | -13.331                  | 75.055                   | 58.171                   | -13.331                  | 95.890                   | 1.710                           | 0.659                         | 0.560                                     | 55.200                                                               | 58.100                                                            |
| BS6  | 207         | 25/07/2016               | 22:05           | bow shock | out    |       | 1.201                    | -109.406                 | -10.023                  | 87.577                   | 65.585                   | -10.023                  | 109.870                  | 1.662                           | 0.643                         | 0.392                                     | 59.800                                                               | 67.500                                                            |
| BS7  | 207         | 25/07/2016               | 22:50           | bow shock | in     |       | 1.197                    | -109.445                 | -10.005                  | 107.911                  | 18.300                   | -10.005                  | 109.908                  | 1.662                           | 0.168                         | 0.392                                     | 59.800                                                               | 67.500                                                            |
| BS8  | 209         | 27/07/2016               | 09:34           | bow shock | out    |       | 1.005                    | -111.026                 | -9.178                   | -109.614                 | -17.680                  | -9.178                   | 111.409                  | 1.653                           | -2.982                        | 0.378                                     | 60.300                                                               | 68.400                                                            |
| BS9  | 209         | 27/07/2016               | 09:37           | bow shock | in     |       | 1.005                    | -111.026                 | -9.178                   | -109.614                 | -17.680                  | -9.178                   | 111.409                  | 1.653                           | -2.982                        | 0.378                                     | 60.300                                                               | 68.400                                                            |
| BS10 | 209         | 27/07/2016               | 09:47           | bow shock | out    |       | 1.004                    | -111.033                 | -9.174                   | -110.873                 | -6.038                   | -9.174                   | 111.416                  | 1.653                           | -3.087                        | 0.378                                     | 60.300                                                               | 68.400                                                            |
| BS11 | 209         | 27/07/2016               | 11:38           | bow shock | in     |       | 0.993                    | -111.107                 | -9.128                   | -44.475                  | 101.822                  | -9.128                   | 111.486                  | 1.653                           | 1.983                         | 0.377                                     | 60.300                                                               | 68.500                                                            |
| BS12 | 209         | 27/07/2016               | 11:45           | bow shock | out    |       | 0.993                    | -111.110                 | -9.126                   | -39.045                  | 104.029                  | -9.126                   | 111.489                  | 1.653                           | 1.930                         | 0.377                                     | 60.300                                                               | 68.500                                                            |
| BS13 | 209         | 27/07/2016               | 11:51           | bow shock | in     |       | 0.992                    | -111.114                 | -9.124                   | -33.506                  | 105.946                  | -9.124                   | 111.492                  | 1.653                           | 1.877                         | 0.377                                     | 60.300                                                               | 68.500                                                            |
| BS14 | 209         | 27/07/2016               | 23:41           | bow shock | out    |       | 0.925                    | -111.542                 | -8.833                   | 87.504                   | 69.176                   | -8.833                   | 111.895                  | 1.650                           | 0.669                         | 0.374                                     | 60.400                                                               | 68.700                                                            |
| BS15 | 210         | 28/07/2016               | 10:28           | bow shock | in     |       | 0.862                    | -111.890                 | -8.563                   | 111.401                  | 10.488                   | -8.563                   | 112.221                  | 1.647                           | 0.094                         | 0.371                                     | 60.500                                                               | 68.900                                                            |
| BS16 | 210         | 28/07/2016               | 11:11           | bow shock | out    |       | 0.858                    | -111.910                 | -8.546                   | 105.941                  | -36.072                  | -8.546                   | 112.240                  | 1.647                           | -0.328                        | 0.371                                     | 60.500                                                               | 68.900                                                            |
| BS17 | 210         | 28/07/2016               | 11:36           | bow shock | in     |       | 0.855                    | -111.922                 | -8.536                   | 92.882                   | -62.453                  | -8.536                   | 112.251                  | 1.647                           | -0.592                        | 0.371                                     | 60.500                                                               | 68.900                                                            |
| BS18 | 210         | 28/07/2016               | 12:03           | bow shock | out    |       | 0.852                    | -111.937                 | -8.523                   | 68.836                   | -88.274                  | -8.523                   | 112.265                  | 1.647                           | -0.908                        | 0.371                                     | 60.500                                                               | 68.900                                                            |
| BS19 | 210         | 28/07/2016               | 12:10           | bow shock | in     |       | 0.852                    | -111.940                 | -8.521                   | 64.087                   | -91.783                  | -8.521                   | 112.267                  | 1.647                           | -0.961                        | 0.371                                     | 60.500                                                               | 68.900                                                            |
| BS20 | 210         | 28/07/2016               | 17:57           | bow shock | out    |       | 0.818                    | -112.104                 | -8.376                   | -12.417                  | 111.418                  | -8.376                   | 112.420                  | 1.645                           | 1.682                         | 0.369                                     | 60.600                                                               | 69.000                                                            |
| BS21 | 210         | 28/07/2016               | 20:39           | bow shock | in     |       | 0.802                    | -112.179                 | -8.307                   | 111.985                  | -6.633                   | -8.307                   | 112.488                  | 1.645                           | -0.059                        | 0.369                                     | 60.600                                                               | 69.100                                                            |
| BS22 | 210         | 28/07/2016               | 20:56           | bow shock | out    |       | 0.801                    | -112.185                 | -8.301                   | 109.547                  | -24.201                  | -8.301                   | 112.495                  | 1.645                           | -0.217                        | 0.369                                     | 60.600                                                               | 69.100                                                            |
| BS23 | 210         | 28/07/2016               | 21:02           | bow shock | in     |       | 0.800                    | -112.188                 | -8.298                   | 108.120                  | -29.945                  | -8.298                   | 112.497                  | 1.645                           | -0.270                        | 0.369                                     | 60.600                                                               | 69.100                                                            |
| BS24 | 221         | 08/08/2016               | 01:39           | bow shock | out    |       | -0.668                   | -108.077                 | -1.528                   | -36.783                  | 101.627                  | -1.528                   | 108.090                  | 1.585                           | 1.918                         | 0.429                                     | 58.600                                                               | 65.100                                                            |
| BS25 | 221         | 08/08/2016               | 03:39           | bow shock | in     |       | -0.679                   | -107.953                 | -1.469                   | 85.816                   | 65.499                   | -1.469                   | 107.966                  | 1.584                           | 0.652                         | 0.430                                     | 58.600                                                               | 65.000                                                            |
| BS26 | 221         | 08/08/2016               | 22:40           | bow shock | out    |       | -0.782                   | -106.705                 | -0.914                   | 39.664                   | 99.062                   | -0.914                   | 106.712                  | 1.579                           | 1.190                         | 0.446                                     | 58.100                                                               | 64.100                                                            |
| BS27 | 222         | 09/08/2016               | 03:22           | bow shock | in     |       | -0.807                   | -106.376                 | -0.777                   | -20.466                  | -104.392                 | -0.777                   | 106.382                  | 1.578                           | -1.764                        | 0.450                                     | 58.000                                                               | 63.900                                                            |
| BS28 | 222         | 09/08/2016               | 16:02           | bow shock | out    |       | -0.873                   | -105.442                 | -0.406                   | -98.741                  | 36.999                   | -0.406                   | 105.446                  | 1.575                           | 2.783                         | 0.462                                     | 57.700                                                               | 63.200                                                            |
| BS29 | 222         | 09/08/2016               | 20:37           | bow shock | in     |       | -0.896                   | -105.088                 | -0.271                   | 104.355                  | -12.424                  | -0.271                   | 105.092                  | 1.573                           | -0.118                        | 0.467                                     | 57.500                                                               | 62.900                                                            |
| BS30 | 222         | 09/08/2016               | 23:10           | bow shock | out    |       | -0.909                   | -104.885                 | -0.195                   | -19.102                  | -103.135                 | -0.195                   | 104.889                  | 1.573                           | -1.754                        | 0.470                                     | 57.500                                                               | 62.700                                                            |
| BS31 | 223         | 10/08/2016               | 19:45           | bow shock | in     |       | -1.009                   | -103.166                 | 0.408                    | -62.229                  | -82.291                  | 0.408                    | 103.172                  | 1.567                           | -2.218                        | 0.493                                     | 56.900                                                               | 61.500                                                            |
| BS32 | 223         | 10/08/2016               | 21:56           | bow shock | out    |       | -1.019                   | -102.975                 | 0.472                    | -92.803                  | 44.637                   | 0.472                    | 102.981                  | 1.566                           | 2.693                         | 0.495                                     | 56.800                                                               | 61.300                                                            |
| BS33 | 223         | 10/08/2016               | 23:39           | bow shock | in     |       | -1.027                   | -102.819                 | 0.523                    | -1.502                   | 102.813                  | 0.523                    | 102.825                  | 1.566                           | 1.585                         | 0.497                                     | 56.700                                                               | 61.200                                                            |
| BS34 | 223         | 10/08/2016               | 23:49           | bow shock | out    |       | -1.028                   | -102.804                 | 0.528                    | 9.333                    | 102.384                  | 0.528                    | 102.810                  | 1.566                           | 1.480                         | 0.498                                     | 56.700                                                               | 61.200                                                            |
| BS35 | 224         | 11/08/2016               | 00:03           | bow shock | in     |       | -1.029                   | -102.781                 | 0.535                    | 25.348                   | 99.612                   | 0.535                    | 102.788                  | 1.566                           | 1.322                         | 0.498                                     | 56.700                                                               | 61.200                                                            |
| BS36 | 224         | 11/08/2016               | 00:12           | bow shock | out    |       | -1.029                   | -102.774                 | 0.538                    | 30.563                   | 98.130                   | 0.538                    | 102.781                  | 1.566                           | 1.269                         | 0.498                                     | 56.700                                                               | 61.200                                                            |
| BS37 | 224         | 11/08/2016               | 01:38           | bow shock | in     |       | -1.036                   | -102.639                 | 0.582                    | 97.457                   | 32.216                   | 0.582                    | 102.646                  | 1.565                           | 0.319                         | 0.500                                     | 56.700                                                               | 61.100                                                            |
| BS38 | 316         | 11/11/2016               | 02:36           | bow shock | out    |       | -14.518                  | -109.325                 | -12.489                  | -109.974                 | 8.265                    | -12.489                  | 110.989                  | 1.684                           | 3.067                         | 0.550                                     | 55.400                                                               | 58.500                                                            |
| BS39 | 316         | 11/11/2016               | 02:42           | bow shock | in     |       | -14.519                  | -109.328                 | -12.487                  | -109.388                 | 14.053                   | -12.487                  | 110.992                  | 1.684                           | 3.014                         | 0.550                                     | 55.400                                                               | 58.500                                                            |
| BS40 | 316         | 11/11/2016               | 02:58           | bow shock | out    |       | -14.523                  | -109.340                 | -12.479                  | -104.030                 | 36.658                   | -12.479                  | 111.004                  | 1.683                           | 2.803                         | 0.550                                     | 55.500                                                               | 58.500                                                            |
| BS41 | 316         | 11/11/2016               | 04:17           | bow shock | in     |       | -14.537                  | -109.385                 | -12.450                  | -47.067                  | 99.805                   | -12.450                  | 111.047                  | 1.683                           | 2.011                         | 0.550                                     | 55.500                                                               | 58.500                                                            |
| BS42 | 316         | 11/11/2016               | 04:18           | bow shock | out    |       | -14.538                  | -109.388                 | -12.448                  | -41.740                  | 102.151                  | -12.448                  | 111.050                  | 1.683                           | 1.959                         | 0.550                                     | 55.500                                                               | 58.500                                                            |
| BS43 | 316         | 11/11/2016               | 04:47           | bow shock | in     |       | -14.542                  | -109.403                 | -12.438                  | -13.664                  | 109.516                  | -12.438                  | 111.064                  | 1.683                           | 1.695                         | 0.550                                     | 55.500                                                               | 58.500                                                            |
| BS44 | 316         | 11/11/2016               | 04:49           | bow shock | out    |       | -14.543                  | -109.406                 | -12.436                  | -7.870                   | 110.087                  | -12.436                  | 111.066                  | 1.683                           | 1.642                         | 0.549                                     | 55.500                                                               | 58.600                                                            |
| BS45 | 316         | 11/11/2016               | 05:01           | bow shock | in     |       | -14.545                  | -109.412                 | -12.432                  | 3.768                    | 110.310                  | -12.432                  | 111.072                  | 1.683                           | 1.537                         | 0.549                                     | 55.500                                                               | 58.600                                                            |
| BS46 | 316         | 11/11/2016               | 23:15           | bow shock | out    |       | -14.737                  | -110.004                 | -11.996                  | -92.091                  | 61.945                   | -11.996                  | 111.633                  | 1.678                           | 2.549                         | 0.544                                     | 55.600                                                               | 58.800                                                            |

Supporting Information for “Effect of a magnetosphere compression on Jovian radio emissions: an in situ case study using Juno data”

|      |     |            |       |           |     |  |         |          |         |          |          |         |         |       |        |       |        |        |
|------|-----|------------|-------|-----------|-----|--|---------|----------|---------|----------|----------|---------|---------|-------|--------|-------|--------|--------|
| BS47 | 316 | 11/11/2016 | 23:16 | bow shock | in  |  | -14.737 | -110.004 | -11.996 | -92.091  | 61.945   | -11.996 | 111.633 | 1.678 | 2.549  | 0.544 | 55.600 | 58.800 |
| BS48 | 316 | 11/11/2016 | 23:18 | bow shock | out |  | -14.738 | -110.006 | -11.994 | -88.698  | 66.717   | -11.994 | 111.635 | 1.678 | 2.497  | 0.544 | 55.600 | 58.800 |
| BS49 | 316 | 11/11/2016 | 23:21 | bow shock | in  |  | -14.738 | -110.006 | -11.994 | -88.698  | 66.717   | -11.994 | 111.635 | 1.678 | 2.497  | 0.544 | 55.600 | 58.800 |
| BS50 | 328 | 23/11/2016 | 16:49 | bow shock | out |  | -15.604 | -104.129 | -3.950  | 102.842  | 22.579   | -3.950  | 105.365 | 1.608 | 0.216  | 0.659 | 53.200 | 53.600 |
| BS51 | 328 | 23/11/2016 | 16:54 | bow shock | in  |  | -15.603 | -104.123 | -3.948  | 103.884  | 17.123   | -3.948  | 105.360 | 1.608 | 0.163  | 0.659 | 53.200 | 53.600 |
| BS52 | 2   | 02/01/2017 | 16:31 | bow shock | out |  | -21.884 | -107.383 | -14.393 | -59.777  | 91.852   | -14.393 | 110.532 | 1.701 | 2.148  | 0.672 | 53.000 | 53.100 |
| BS53 | 2   | 02/01/2017 | 17:39 | bow shock | in  |  | -21.901 | -107.429 | -14.367 | 17.646   | 108.209  | -14.367 | 110.576 | 1.701 | 1.409  | 0.671 | 53.000 | 53.100 |
| BS54 | 3   | 03/01/2017 | 03:40 | bow shock | out |  | -22.039 | -107.794 | -14.138 | 22.849   | 107.626  | -14.138 | 110.929 | 1.699 | 1.362  | 0.667 | 53.000 | 53.300 |
| BS55 | 3   | 03/01/2017 | 20:25 | bow shock | in  |  | -22.254 | -108.328 | -13.745 | -108.755 | -20.061  | -13.745 | 111.441 | 1.694 | -2.959 | 0.661 | 53.200 | 53.500 |
| BS56 | 4   | 04/01/2017 | 00:08 | bow shock | out |  | -22.300 | -108.433 | -13.655 | 64.396   | 90.046   | -13.655 | 111.542 | 1.694 | 0.950  | 0.660 | 53.200 | 53.600 |
| BS57 | 4   | 04/01/2017 | 02:09 | bow shock | in  |  | -22.323 | -108.488 | -13.607 | 105.271  | -34.438  | -13.607 | 111.594 | 1.693 | -0.316 | 0.659 | 53.200 | 53.600 |
| BS58 | 11  | 11/01/2017 | 13:05 | bow shock | out |  | -23.300 | -107.715 | -8.679  | 97.437   | -51.494  | -8.679  | 110.548 | 1.649 | -0.486 | 0.696 | nan    | nan    |
| BS59 | 11  | 11/01/2017 | 15:16 | bow shock | in  |  | -23.297 | -107.637 | -8.613  | -31.179  | -105.624 | -8.613  | 110.466 | 1.649 | -1.858 | 0.697 | nan    | nan    |
| BS60 | 11  | 11/01/2017 | 15:17 | bow shock | out |  | -23.297 | -107.637 | -8.613  | -31.179  | -105.624 | -8.613  | 110.466 | 1.649 | -1.858 | 0.697 | nan    | nan    |
| BS61 | 11  | 11/01/2017 | 15:20 | bow shock | in  |  | -23.297 | -107.634 | -8.610  | -36.704  | -103.830 | -8.610  | 110.463 | 1.649 | -1.911 | 0.697 | nan    | nan    |
| BS62 | 11  | 11/01/2017 | 15:40 | bow shock | out |  | -23.297 | -107.622 | -8.600  | -57.632  | -93.828  | -8.600  | 110.450 | 1.649 | -2.122 | 0.698 | nan    | nan    |
| BS63 | 11  | 11/01/2017 | 19:38 | bow shock | in  |  | -23.290 | -107.472 | -8.477  | -6.427   | 109.779  | -8.477  | 110.293 | 1.648 | 1.629  | 0.700 | nan    | nan    |
| BS64 | 11  | 11/01/2017 | 21:09 | bow shock | out |  | -23.287 | -107.414 | -8.431  | 85.486   | 69.082   | -8.431  | 110.233 | 1.647 | 0.680  | 0.702 | nan    | nan    |
| BS65 | 11  | 11/01/2017 | 22:36 | bow shock | in  |  | -23.284 | -107.359 | -8.388  | 107.274  | -23.672  | -8.388  | 110.175 | 1.647 | -0.217 | 0.703 | nan    | nan    |
| BS66 | 12  | 12/01/2017 | 03:34 | bow shock | out |  | -23.273 | -107.159 | -8.233  | -106.489 | 26.169   | -8.233  | 109.966 | 1.646 | 2.901  | 0.707 | nan    | nan    |
| BS67 | 12  | 12/01/2017 | 03:39 | bow shock | in  |  | -23.273 | -107.156 | -8.231  | -104.958 | 31.747   | -8.231  | 109.963 | 1.646 | 2.848  | 0.707 | nan    | nan    |
| BS68 | 12  | 12/01/2017 | 03:47 | bow shock | out |  | -23.273 | -107.152 | -8.228  | -103.134 | 37.236   | -8.228  | 109.958 | 1.646 | 2.795  | 0.707 | nan    | nan    |
| BS69 | 12  | 12/01/2017 | 04:00 | bow shock | in  |  | -23.272 | -107.142 | -8.220  | -95.968  | 53.020   | -8.220  | 109.948 | 1.646 | 2.637  | 0.707 | nan    | nan    |
| BS70 | 12  | 12/01/2017 | 04:30 | bow shock | out |  | -23.271 | -107.121 | -8.205  | -74.682  | 80.244   | -8.205  | 109.926 | 1.646 | 2.320  | 0.707 | nan    | nan    |
| BS71 | 12  | 12/01/2017 | 08:39 | bow shock | in  |  | -23.260 | -106.946 | -8.076  | 103.976  | -34.169  | -8.076  | 109.744 | 1.644 | -0.318 | 0.711 | nan    | nan    |
| BS72 | 12  | 12/01/2017 | 09:14 | bow shock | out |  | -23.258 | -106.921 | -8.057  | 84.614   | -69.380  | -8.057  | 109.718 | 1.644 | -0.687 | 0.711 | nan    | nan    |
| BS73 | 12  | 12/01/2017 | 09:33 | bow shock | in  |  | -23.257 | -106.907 | -8.047  | 68.195   | -85.553  | -8.047  | 109.703 | 1.644 | -0.898 | 0.711 | nan    | nan    |
| BS74 | 12  | 12/01/2017 | 10:57 | bow shock | out |  | -23.253 | -106.849 | -8.006  | -18.621  | -107.753 | -8.006  | 109.643 | 1.644 | -1.742 | 0.713 | nan    | nan    |
| BS75 | 12  | 12/01/2017 | 14:05 | bow shock | in  |  | -23.243 | -106.709 | -7.907  | -89.823  | 62.121   | -7.907  | 109.497 | 1.643 | 2.537  | 0.715 | nan    | nan    |

Supporting Information for “Effect of a magnetosphere compression on Jovian radio emissions: an in situ case study using Juno data”

**File F1 – List of Magnetopause boundary crossings from Juno/Waves and Juno/MAG measurements**

This file (boundary\_crossings\_characteristics\_MP.csv) contains the same information as Table S1, in csv format.

**File F2 – List of bow shock crossings from Juno/Waves and Juno/MAG measurements**

This file (boundary\_crossings\_characteristics\_BS.csv) contains the same information as Table S2, in csv format.

**Figure S1 – 3D projection of the Magnetopause and Bow Shock crossings**

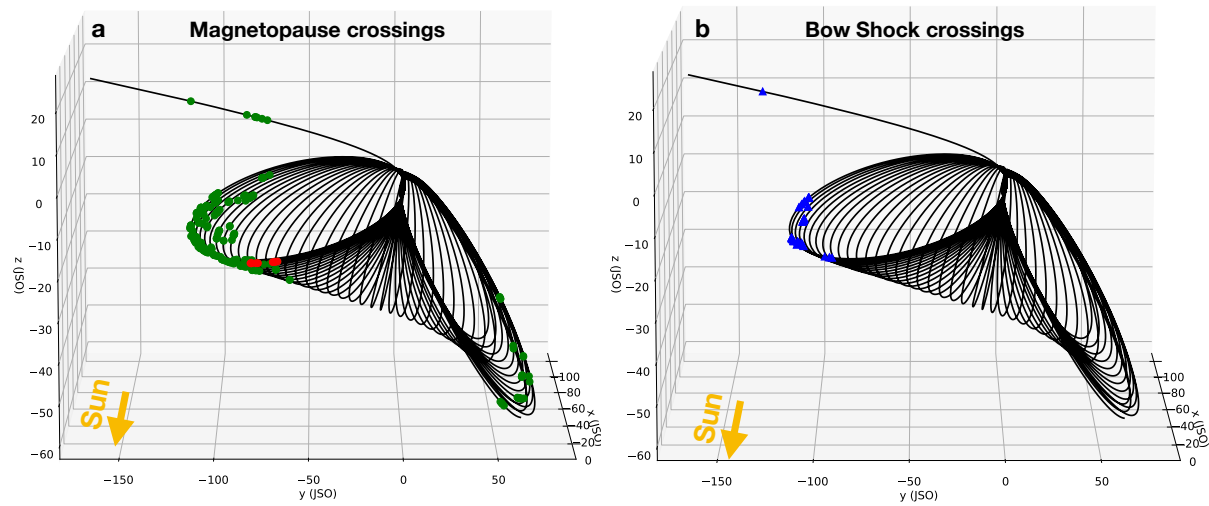

*Figure S1: 3D projection of the Juno trajectory, with the (a) magnetopause and (b) bow-shock crossings overplotted. The magnetopause crossings studied in this article (see Figure 3 in the main article) are highlighted in red in panel (a). The coordinates used here are the Jupiter-Sun-Orbit (JSO) coordinate system. In this system, X is aligned with the Jupiter-Sun vector, Y indicates the Sun's motion in Jupiter frame, and Z close the system.*

**Figure S2 – Statistical distributions based on Magnetosphere boundaries crossings**

Supporting Information for “Effect of a magnetosphere compression on Jovian radio emissions: an in situ case study using Juno data”

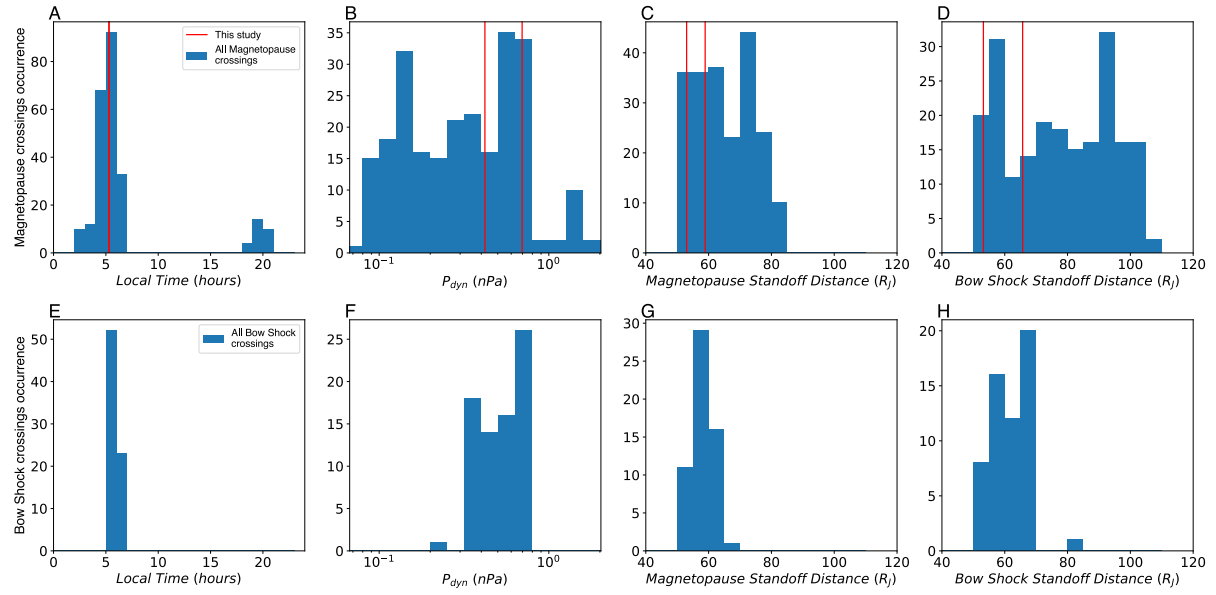

Figure S2: Statistical distributions based on (A-D) magnetopause and (E-H) bow shock crossings. (A,E) Local Time distribution. (B,F) Solar wind dynamic pressure  $P_{dyn}$  distribution. (C,G) Magnetopause standoff distance distribution. (D,H) Bow shock standoff distance distribution. The red lines in panels (A-D) show the position in the distribution of the two compressions studied in the main article.

**Figure S3 – Solar wind characteristics from Tao et al. (2005)’s model**

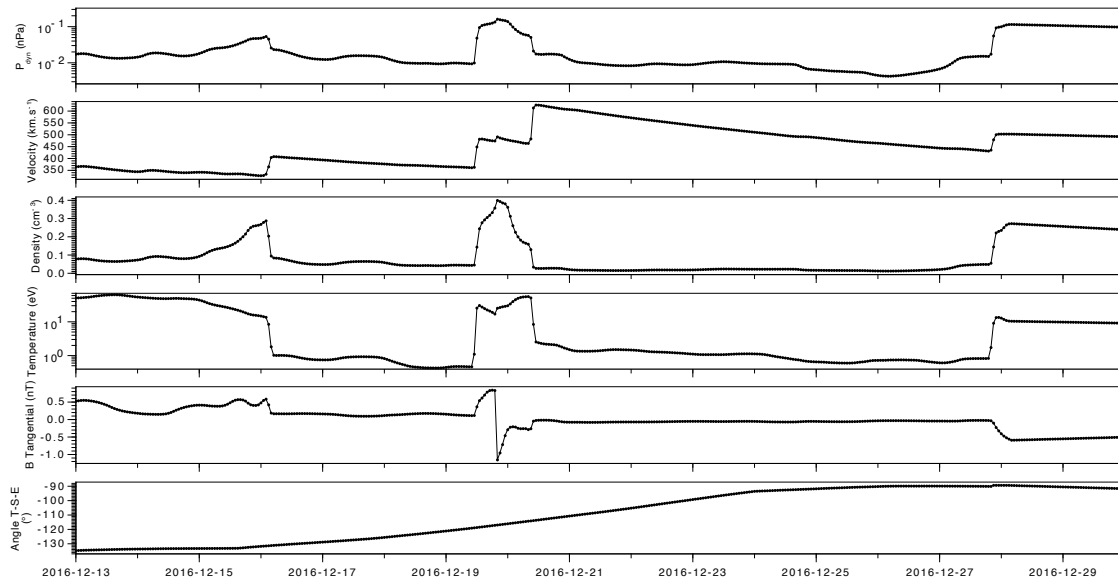

*Figure S3. This Figure displays the Solar Wind characteristics, as calculated by the Tao et al. (2005) model: (i) the Dynamic Pressure  $P_{dyn}$ , (ii) the velocity, (iii) the density, (iv) the temperature, (v) the tangential component of the magnetic field  $B$  and (vi) the Jupiter-Sun-Earth angle.*

**Figure S4 - Solar wind dynamic pressure from Tao et al. (2005)’s model, shifted in time.**

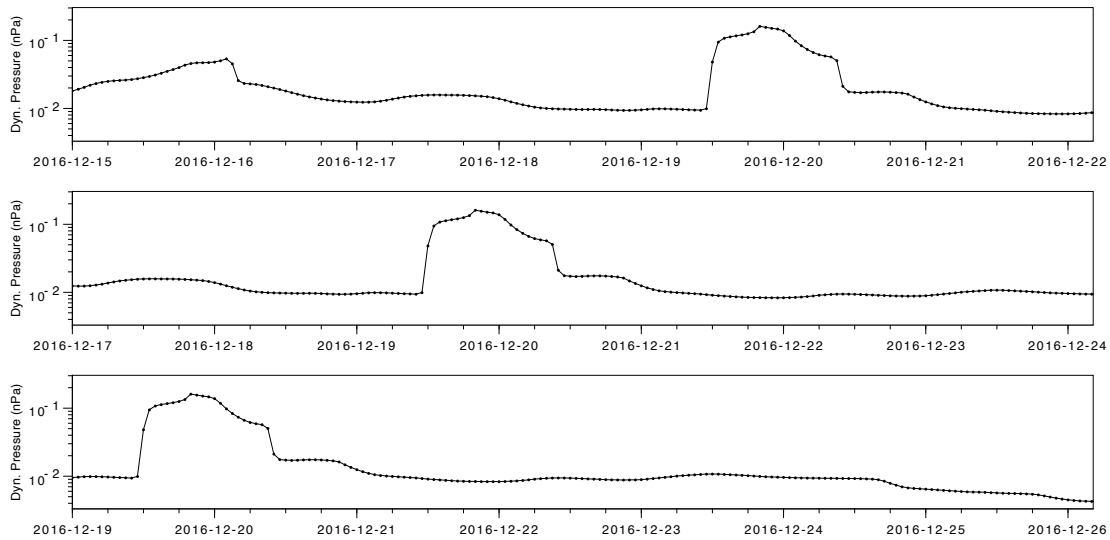

*Figure S4: This Figure displays the Solar Wind Dynamic Pressure  $P_{dyn}$ , as calculated by the Tao et al. (2005) model. Top panel is shifted by minus two day, middle panel is not shifted and bottom panel is shifted by plus two days.*

**Figure S5 - nKOM timeseries at different frequencies.**

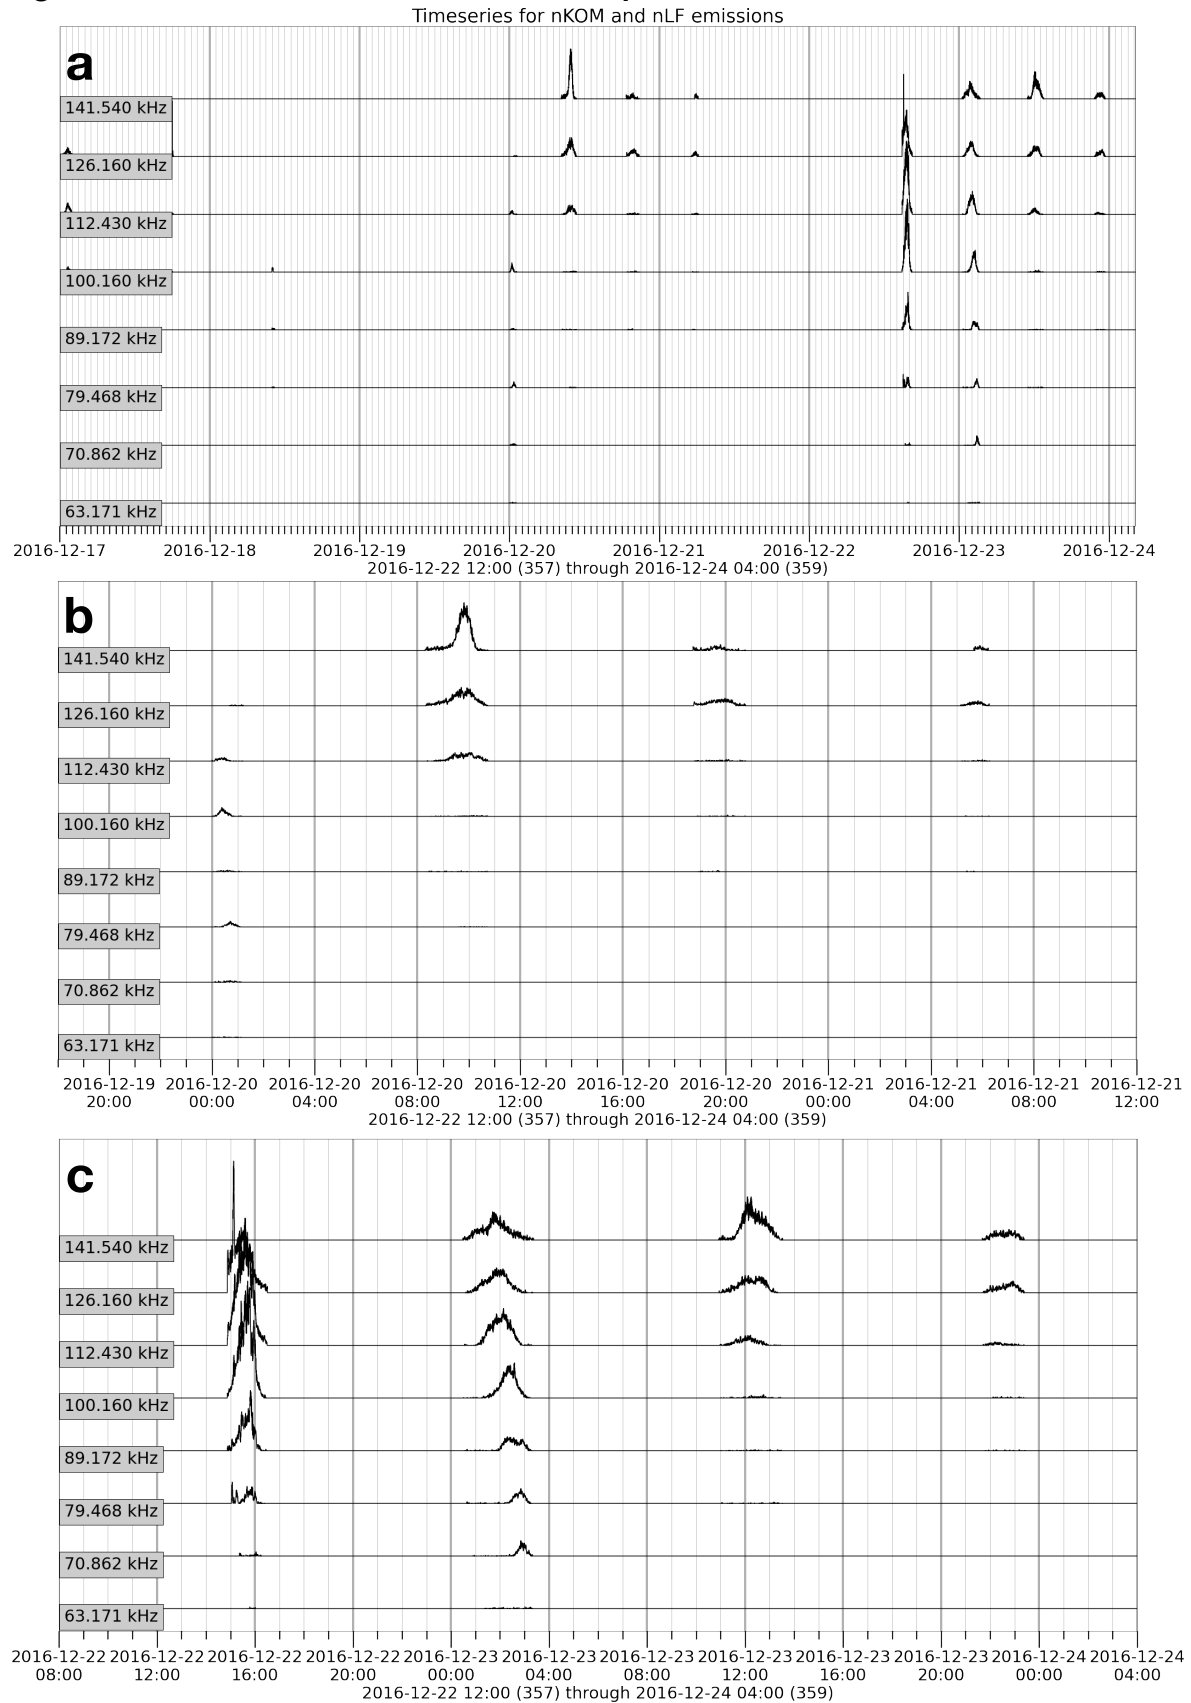

*Figure S3: nKOM time series for all frequency channels in the band where the signal is detected. (a) Same time range than Figure 3. (b) Zoom on the first and (c) second compression. The intensity is normalized to the maximum value measured during the interval studied.*

Supporting Information for “Effect of a magnetosphere compression on Jovian radio emissions: an in situ case study using Juno data”

Figure S4 display time series of narrowband kilometric (nKOM) emissions (measured by Juno/Waves) for all frequency channels where the signal is detected. The scale of the x-axis (time) of the first panel is the same than in Figure 3 of the article. Panels b and c are zooms on the (b) first and (c) second compression. We can clearly see that new nKOM emissions are activated at ~2016-12-20T00:00 and at ~2016-12-22T15:00.

One can see that the activation of sources is not the same at all frequencies. The lower frequencies are triggered before the higher ones, and also disappear first. For example during the second compression (panel c), the 89.172 kHz signal is visible during the first two rotations, while the 141.54 signal is visible during the last 3 rotations.

One can also see during the second compression (panel c) that the centers of signal distribution at different frequencies are shifting over time. During the first rotation, the periodicity is shorter for the higher frequencies than the lower frequencies.
